# Supplementary material for: Adversarial Robustness Guarantees for Classification with Gaussian Processes
Source: arXiv:1905.11876 source file (2020-03-11)
Supplement: Supplementary file 1 [file appendix_algorithm.tex]

In Algorithm \ref{alg:bnb}, we give a more detailed and formal version of Algorithm \ref{alg:bnb_sketch}.

\begin{spacing}{1.1}
\begin{algorithm} 
\caption{Branch and bound for computation of $\piInf{T}$}\label{alg:bnb}
\textbf{Input:} $T$ --- input space subset; $\mu(\cdot), \Sigma(\cdot)$ --- latent mean and variance functions; $\{S_i\}_{i = 1,\ldots, N}$ --- latent space partition; $\epsilon$ --- error tolerance. \\
\textbf{Output:} $\piInfL{T}$ and $\piInfU{T}$ --- lower and upper bounds on $\piInf{T}$, s.t. $\piInfU{T} - \piInfL{T} \leq \epsilon$.
\begin{algorithmic}[1]
\State $\piInfL{T} \gets - \infty $; \quad $\piInfU{T} \gets + \infty $; \quad $\mathbf{R} \gets \{ T \}$
\While{ $\piInfU{T} - \piInfL{T} > \epsilon$}
\State $R \gets$ Select region with current lowest $\piInfL{R}$ for $R \in \mathbf{R}$; \quad $\mathbf{R} \gets \mathbf{R} \setminus R $ 
\State $[\mu^L_R,\mu^U_R] , [\Sigma^L_R\Sigma^U_R] \gets $ Solve Eqn \eqref{eq:mean_variance_bounds} in $R$ for ranges of $\mu(x)$ and $\Sigma(x)$
%\State $[\Sigma^L_R\Sigma^U_R] \gets $ Solve Eqn \eqref{eq:mean_variance_bounds} in $R$ for ranges of $\Sigma(x)$
%\State $\piInfL(R) \gets 0$
\For{$i = 1,\ldots,N$}
\State $\underline{\pi}^L_i(R) \gets $ Compute right-hand side of Eqn \eqref{eq:inf_gauss_int}  (Proposition \ref{Prop:Gaussian})
%\State $\piInfL(R) \gets \piInfL(R) + \sigma (a_i) \piInfL_{R,i} $ \quad --- \quad Application of Proposition \ref{Theorem:BOundsGenericBIclass}
\EndFor
\State $\piInfL{R} \gets $ Apply Proposition \ref{Theorem:BOundsGenericBIclass} to $\{\underline{\pi}^L_i(R)\}_{i=1,\ldots,N}$ and $\{S_i\}_{i=1,\ldots,N}$
\State $\piInfU{R} \gets $ Evaluate GP in candidate optimum.
\If{$\piInfU{R} - \piInfL{R} > \epsilon$}
\State $R_1,R_2 \gets $ Split R in two sub-regions; $\mathbf{R} \gets \mathbf{R} \cup \{R_1,R_2\} $
%\For{j=1,2} Initialize $R_j$ bounds values to $R$ ones. 
%\EndFor
\State $\piInfL{R_j}, \piInfU{R_j} \gets \piInfL{R},\piInfU{R}$ \quad  with $j=1,2$
%\State $\piInfL(R_j)$
\EndIf
%\State $\piInfU(T) \gets \min \left( \piInfU(T), \piInfU(R) \right)$;  $\piInfL(T) \gets \max$ of $\piInfL(R^*)$ for  $R^*$ in $\mathbf{R}$ 
%\If{$\piInfU{R} < \piInfU{T}$}
\State $\piInfL{T},\piInfU{T} \gets$ Update current best bounds
%\EndIf
\EndWhile
%\State $n^C  $
\State \textbf{return} $[\piInfL{T},\piInfU{T}]$
%\WHILE{$ n < n_{\max}$}
%\STATE $w  sample from $p(w | )$
%\\ENDWHILE
%\STATE return $\hat{p}$
\end{algorithmic}
\end{algorithm}
\end{spacing}
