# Supplementary material for: Adversarial Robustness Guarantees for Classification with Gaussian Processes
Source: arXiv:1905.11876 source file (2020-03-11)
Supplement: Supplementary file 2 [file appendix_alternativefigures.tex]

Suggested new version of Robustness figure in Section 6.2:

\begin{figure}
	\centering
	%\includegraphics[width = 0.48\textwidth]{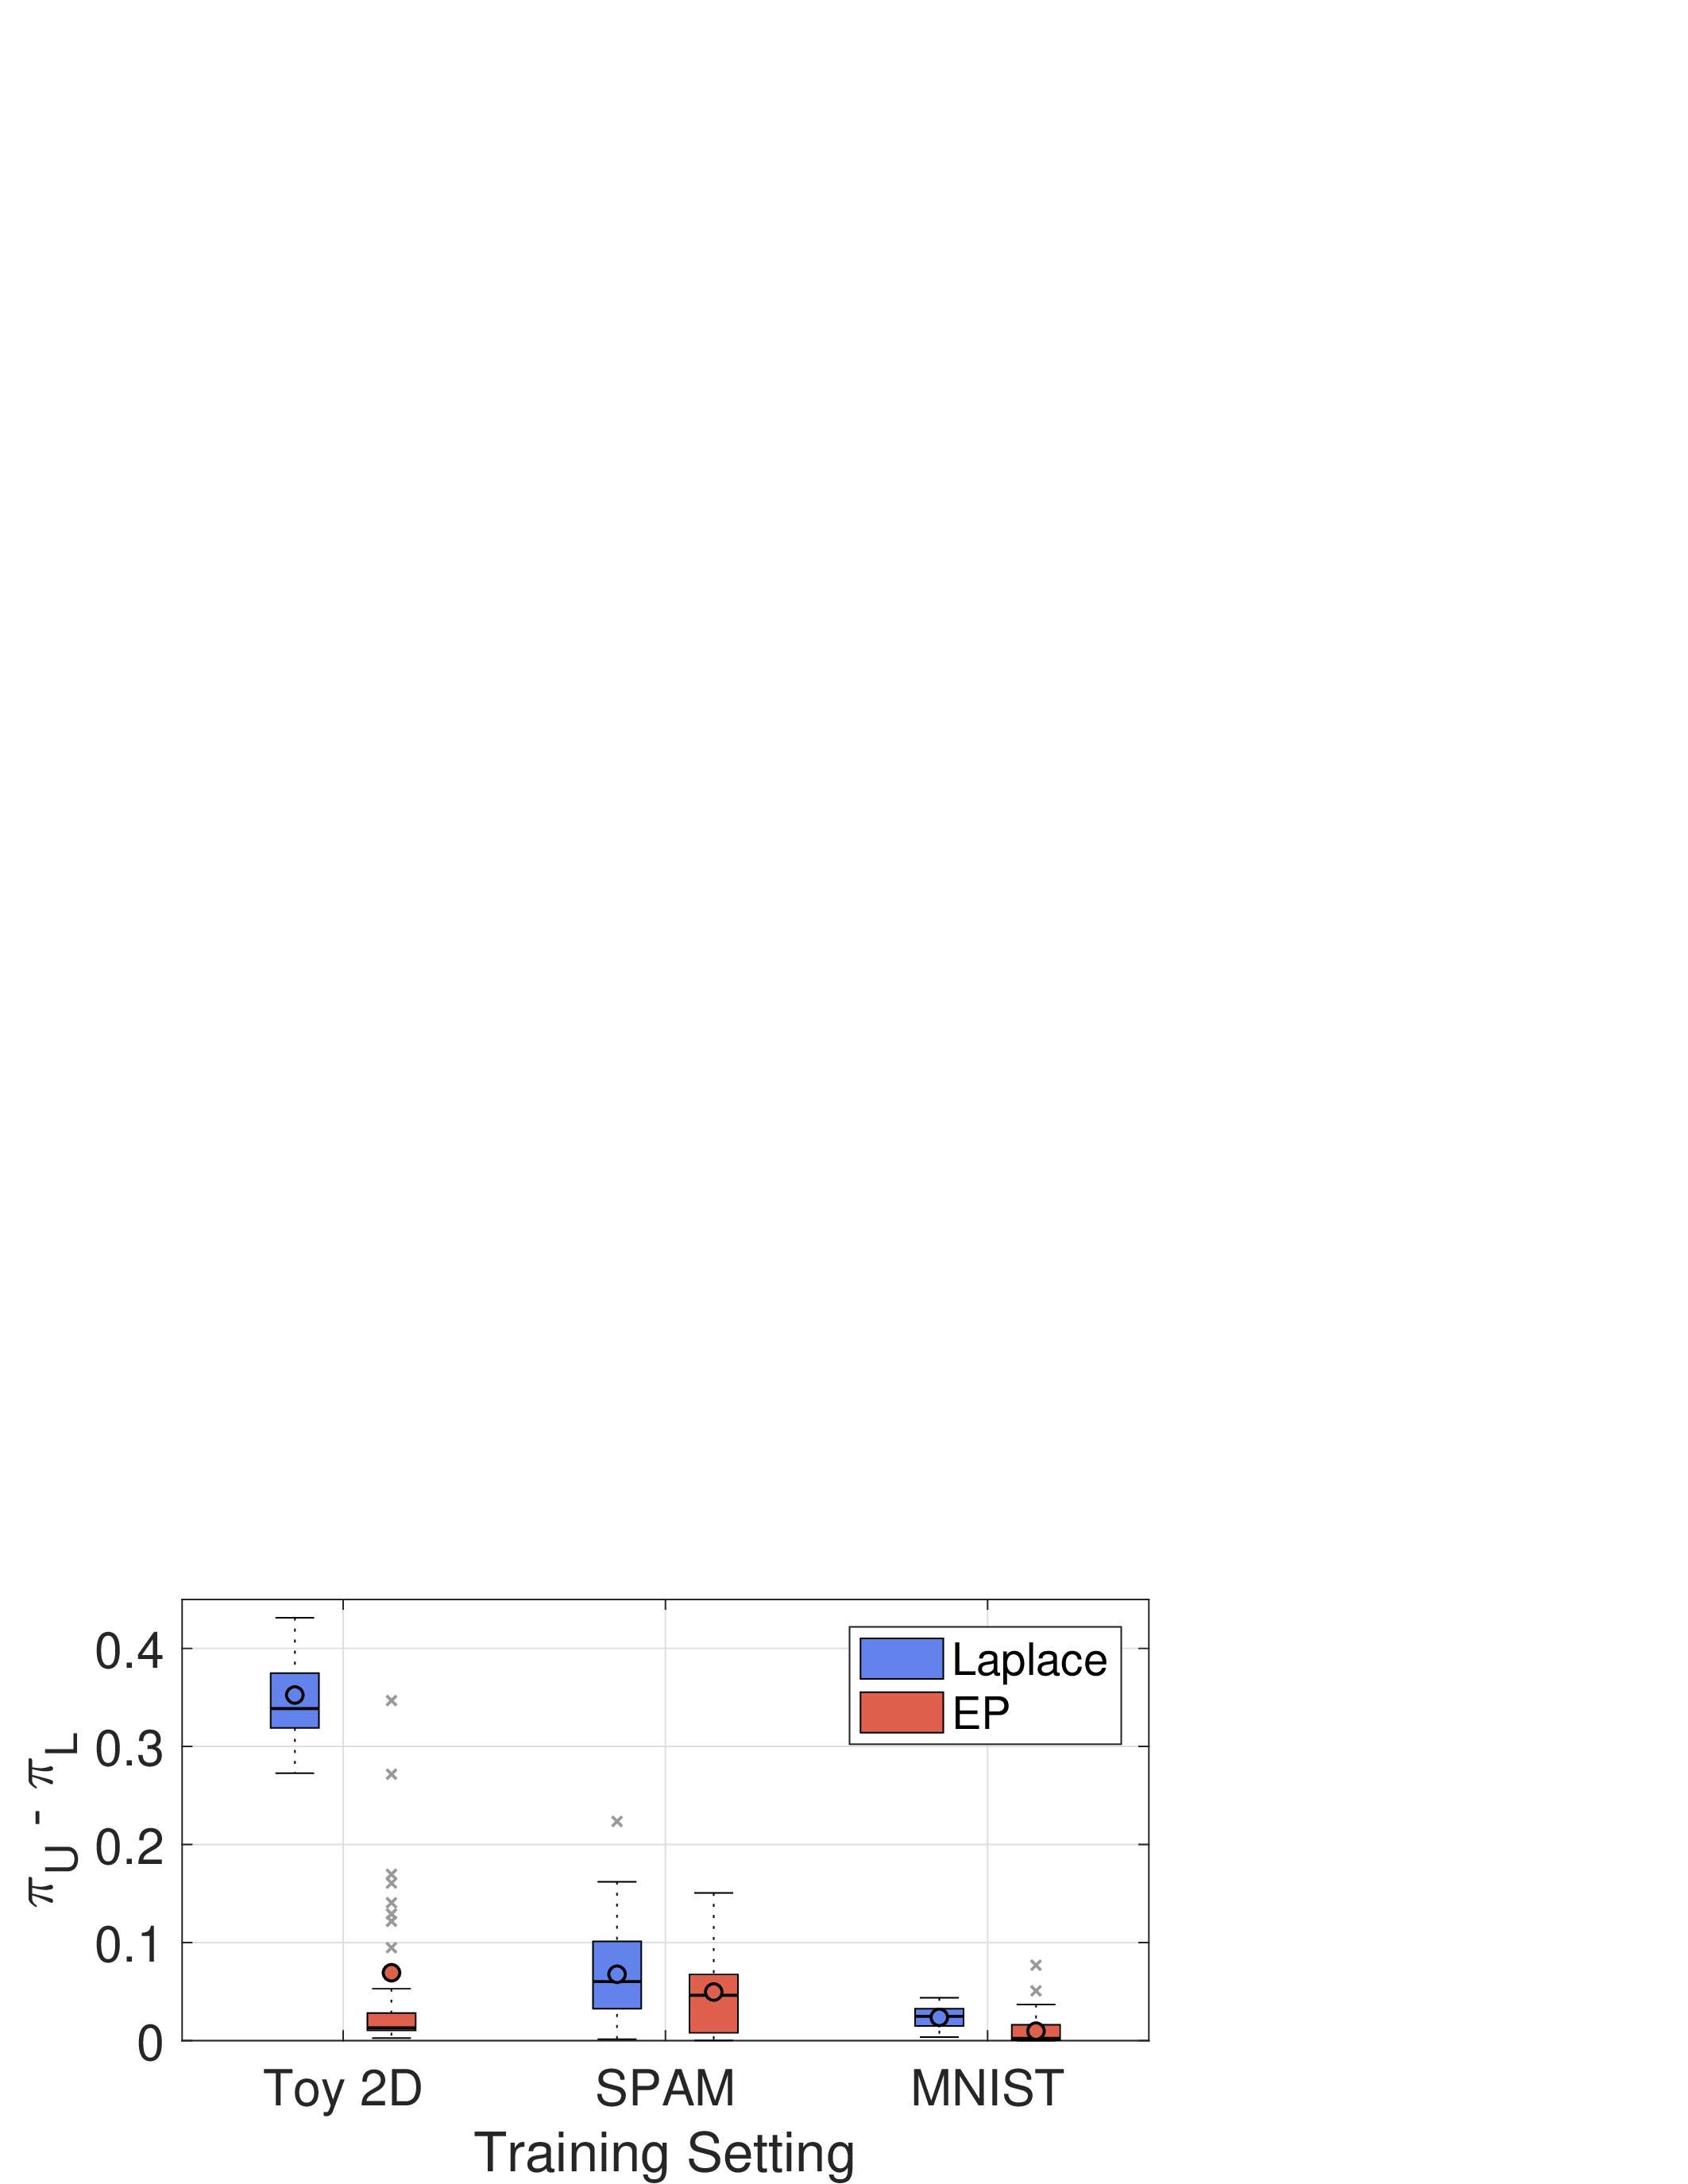}
	%\includegraphics[width = 0.48\textwidth]{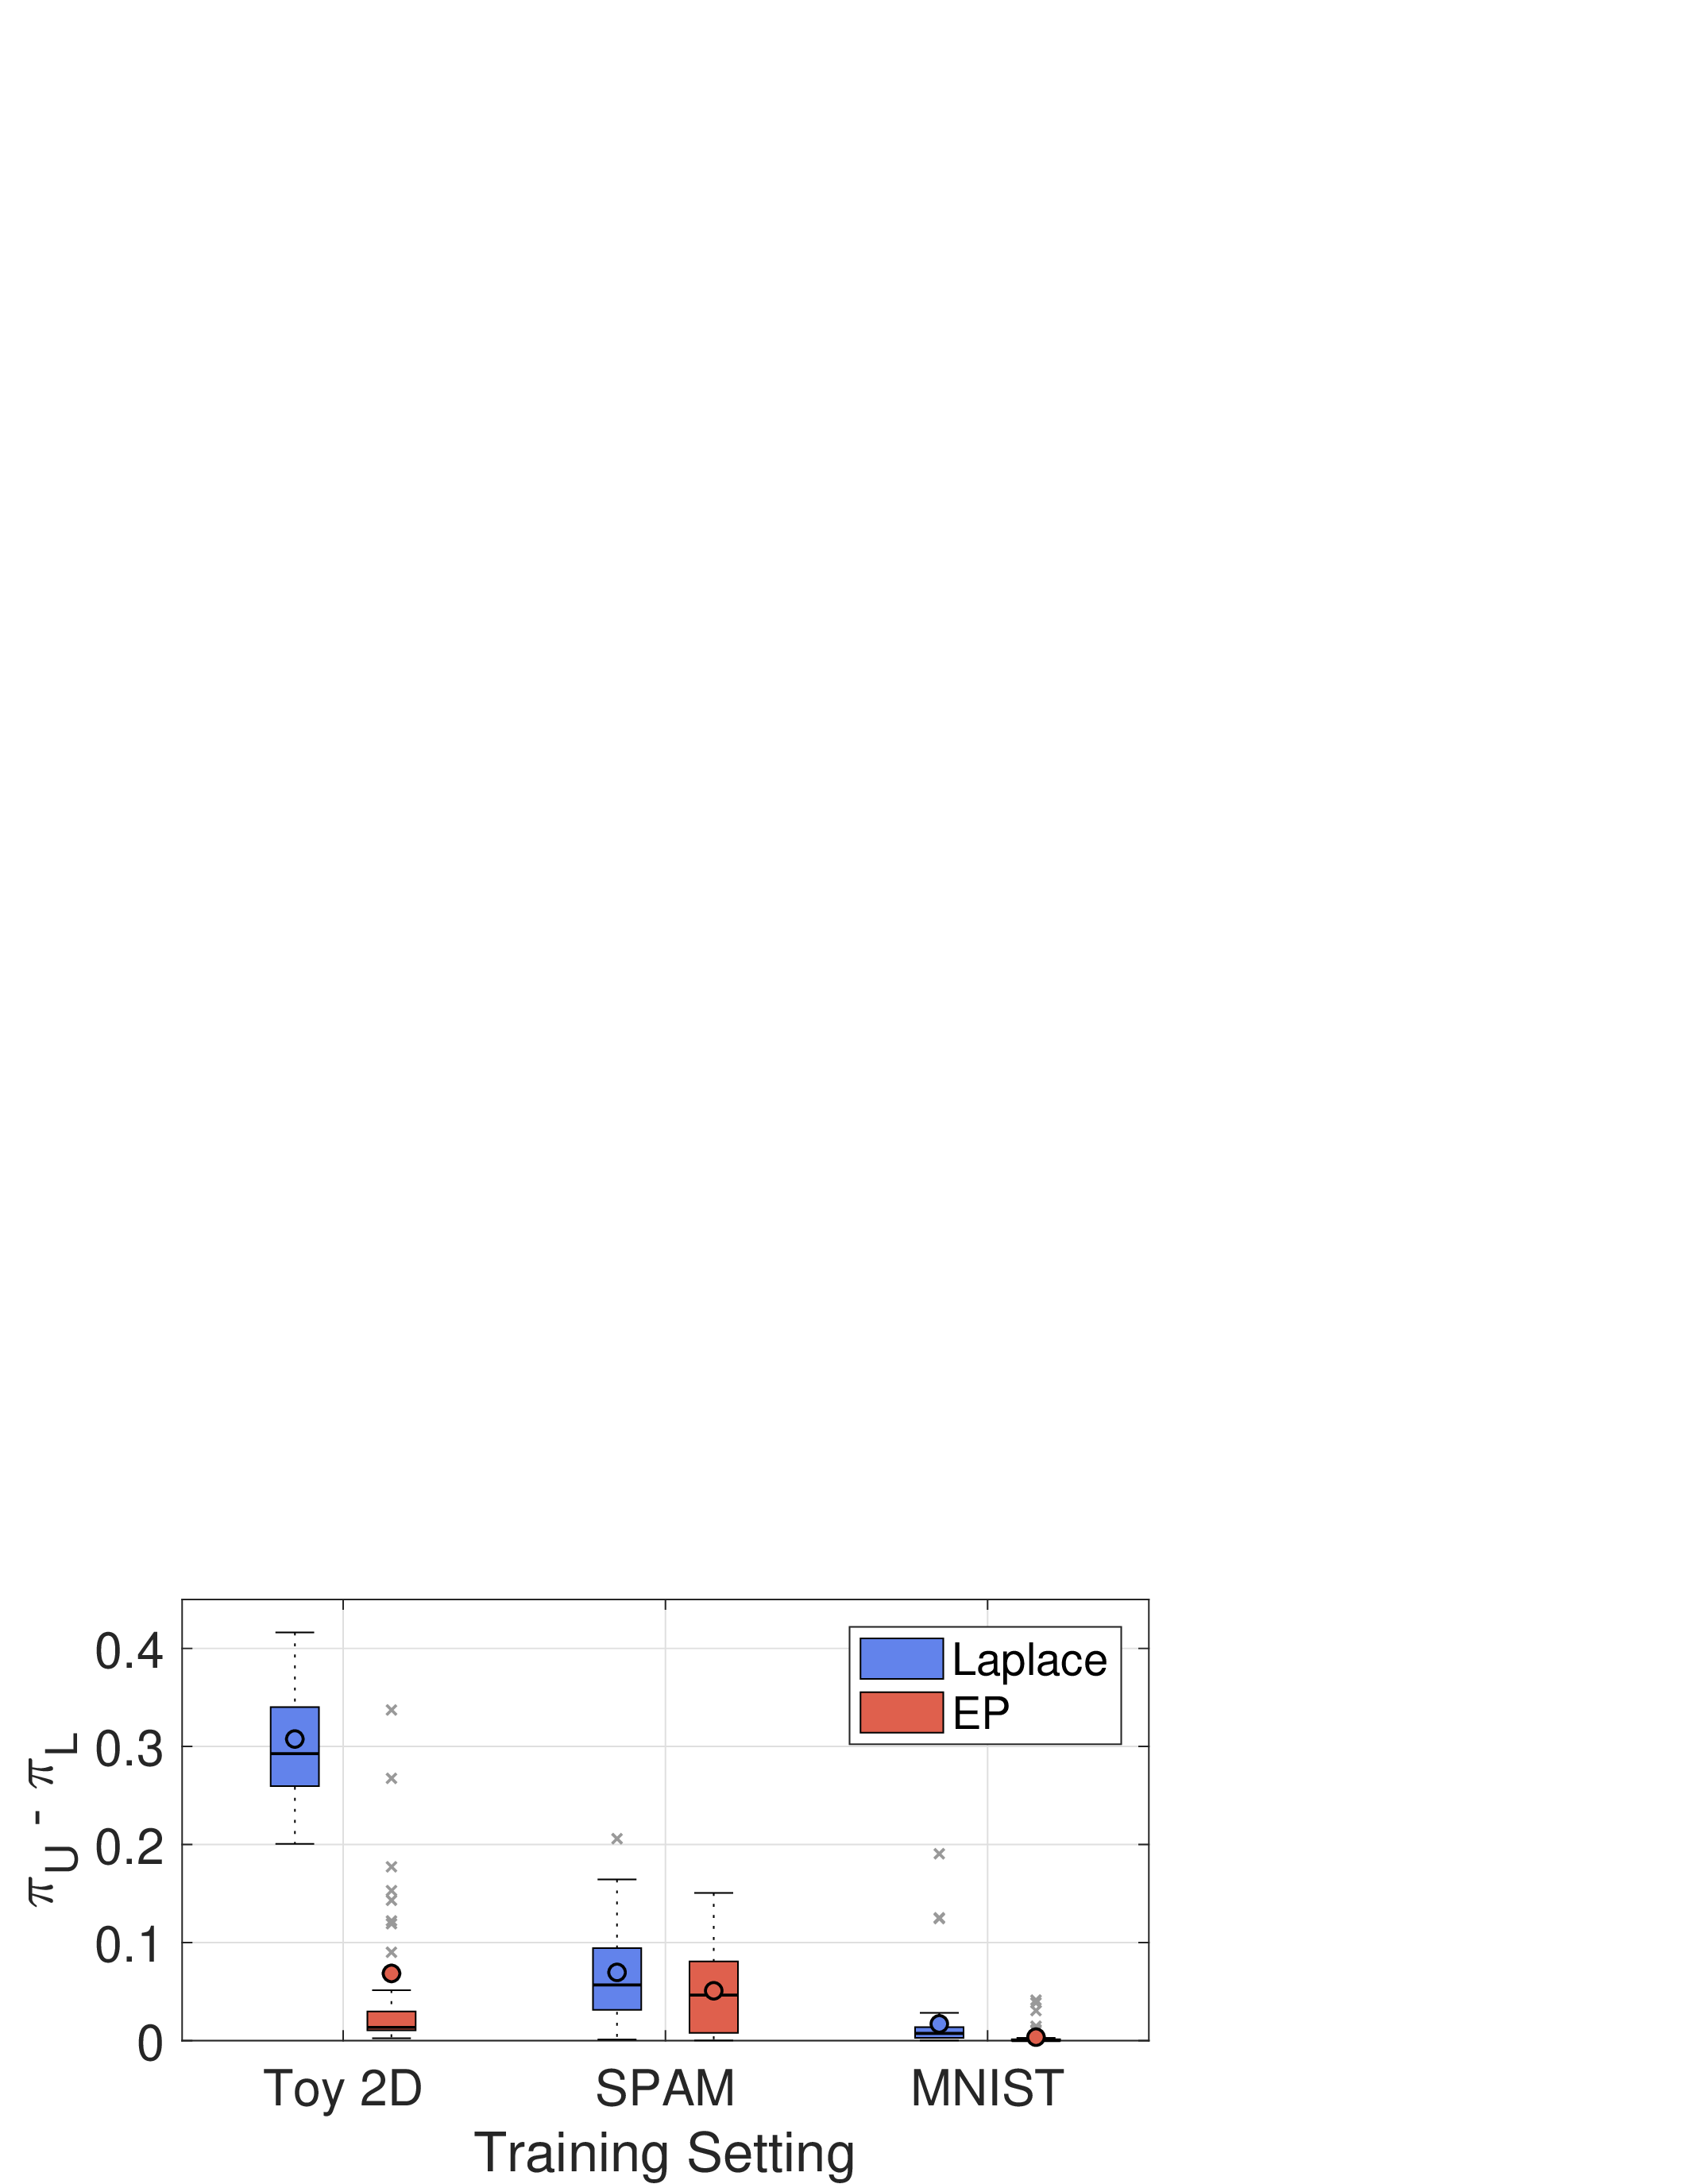}
	
	%% OLD VERSION:
	%\includegraphics[width = 0.49\textwidth]{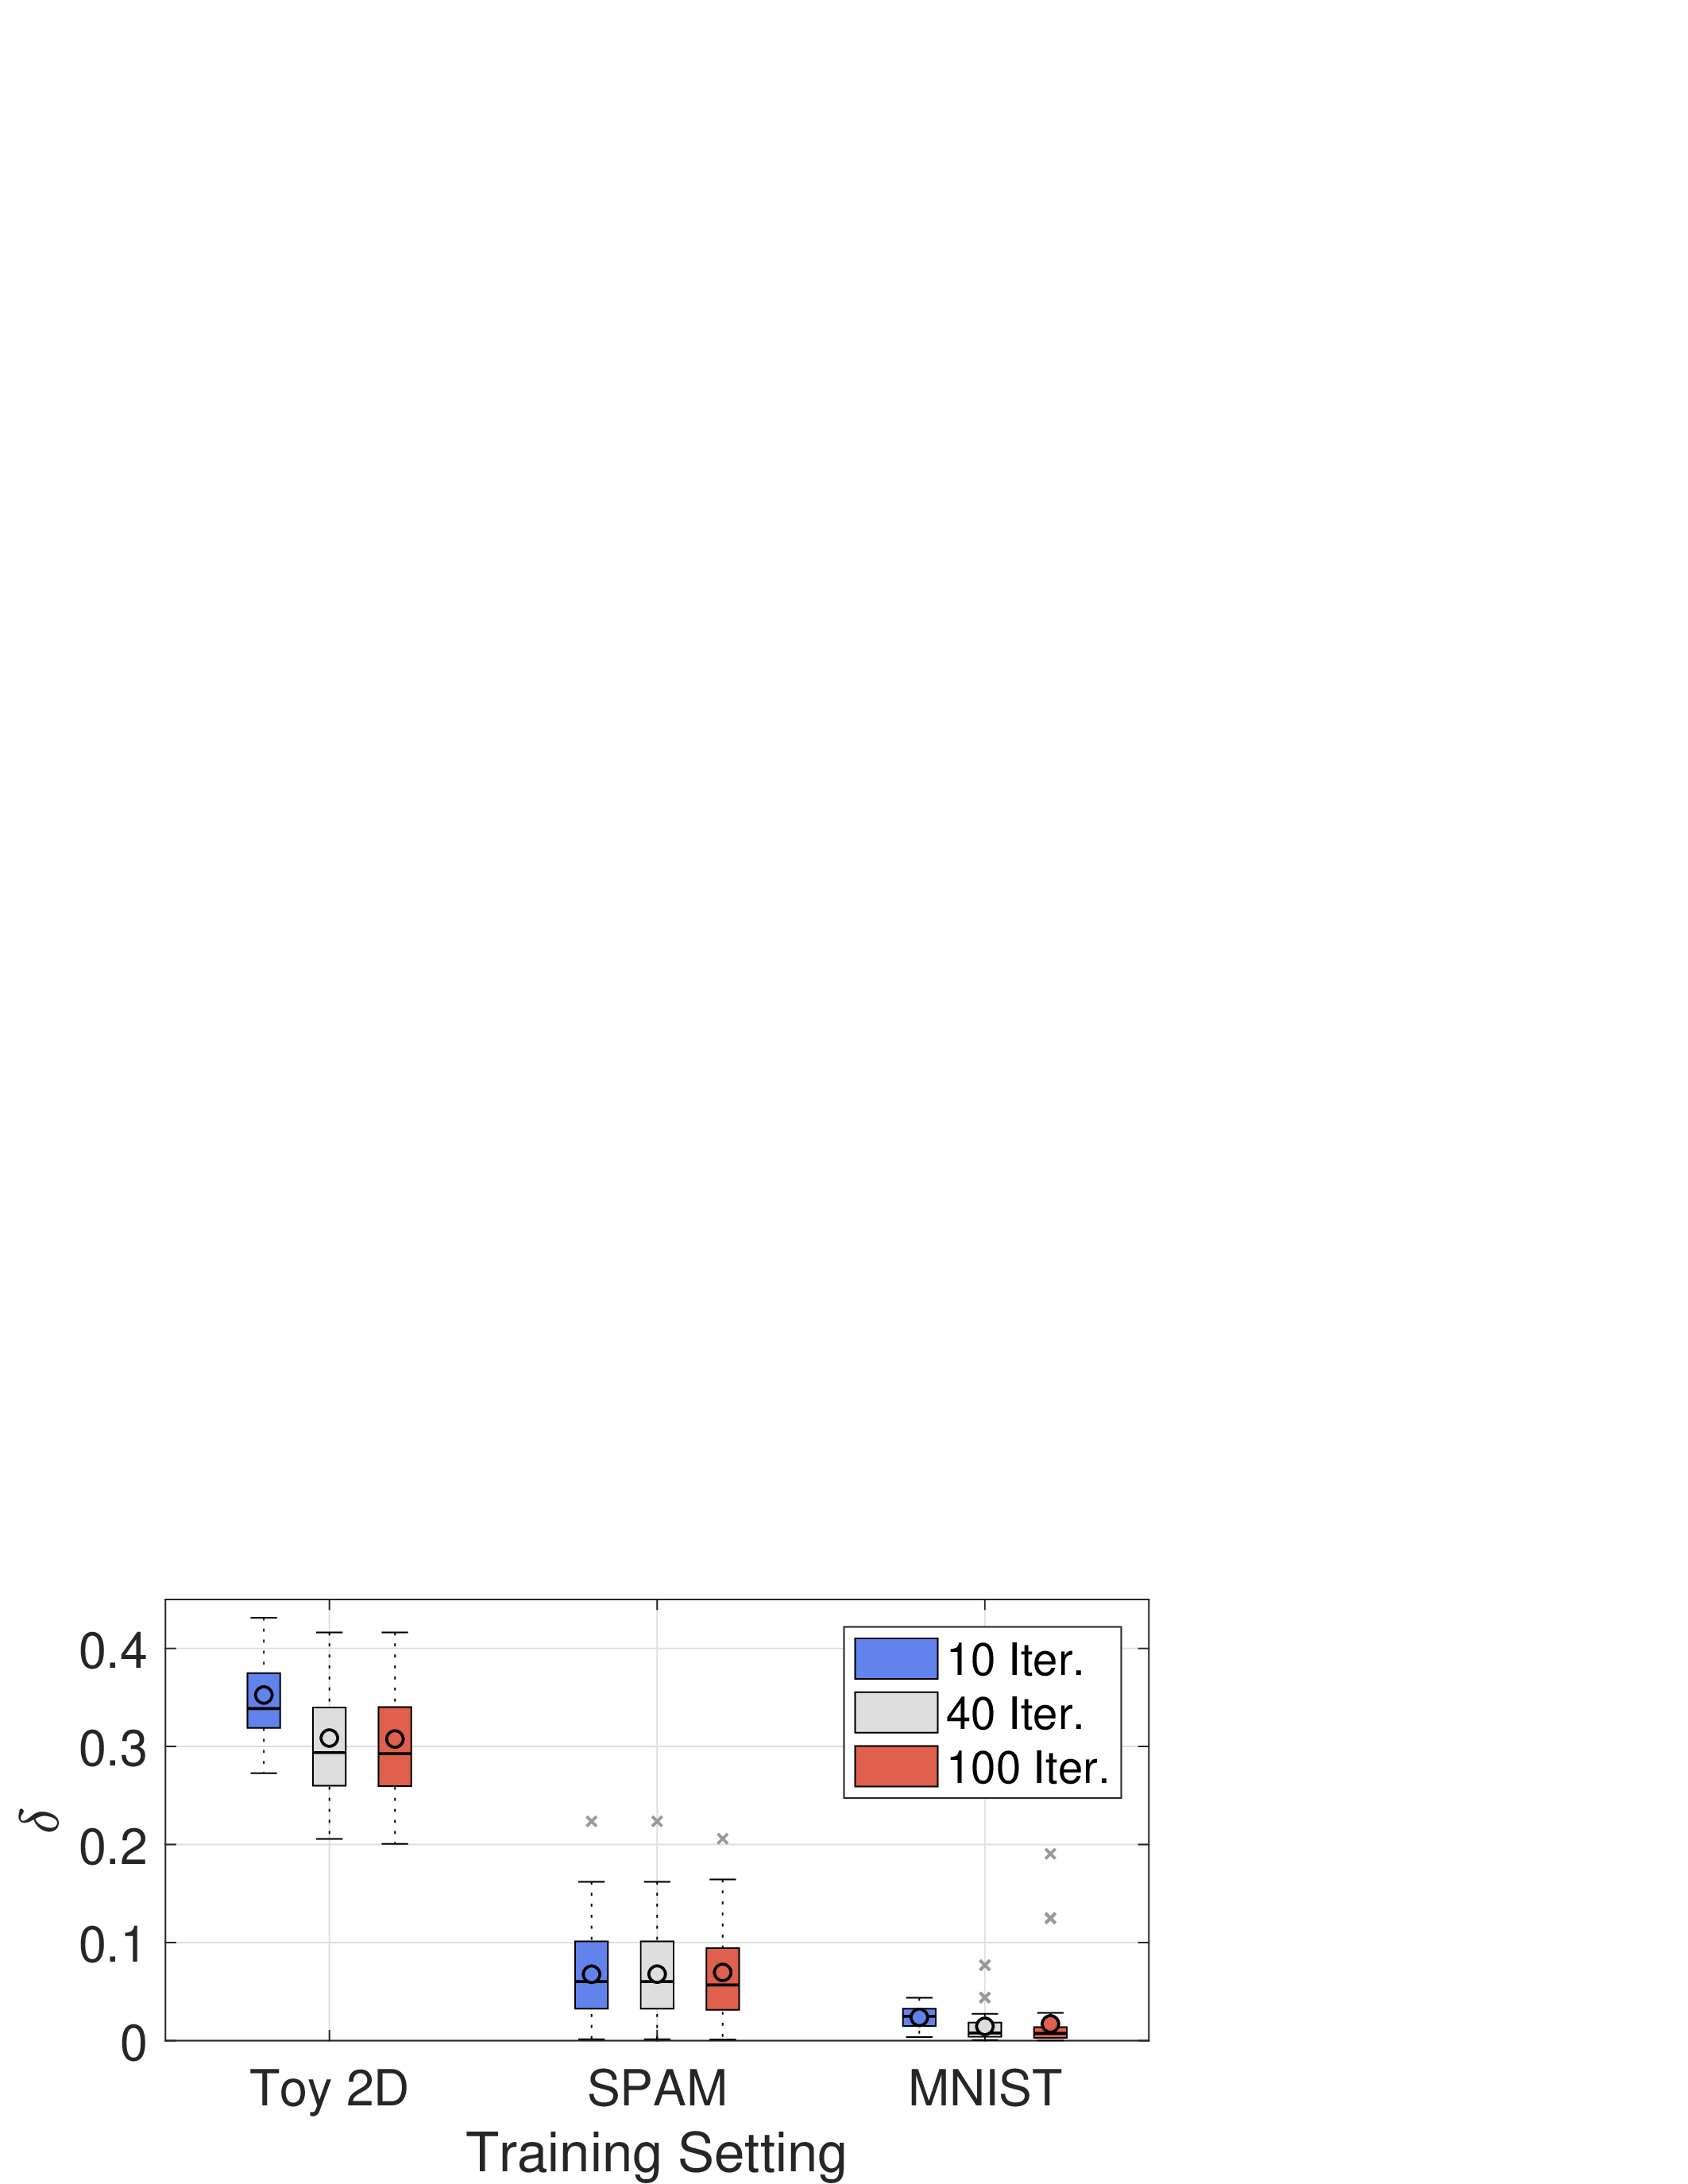}
	%\includegraphics[width = 0.49\textwidth]{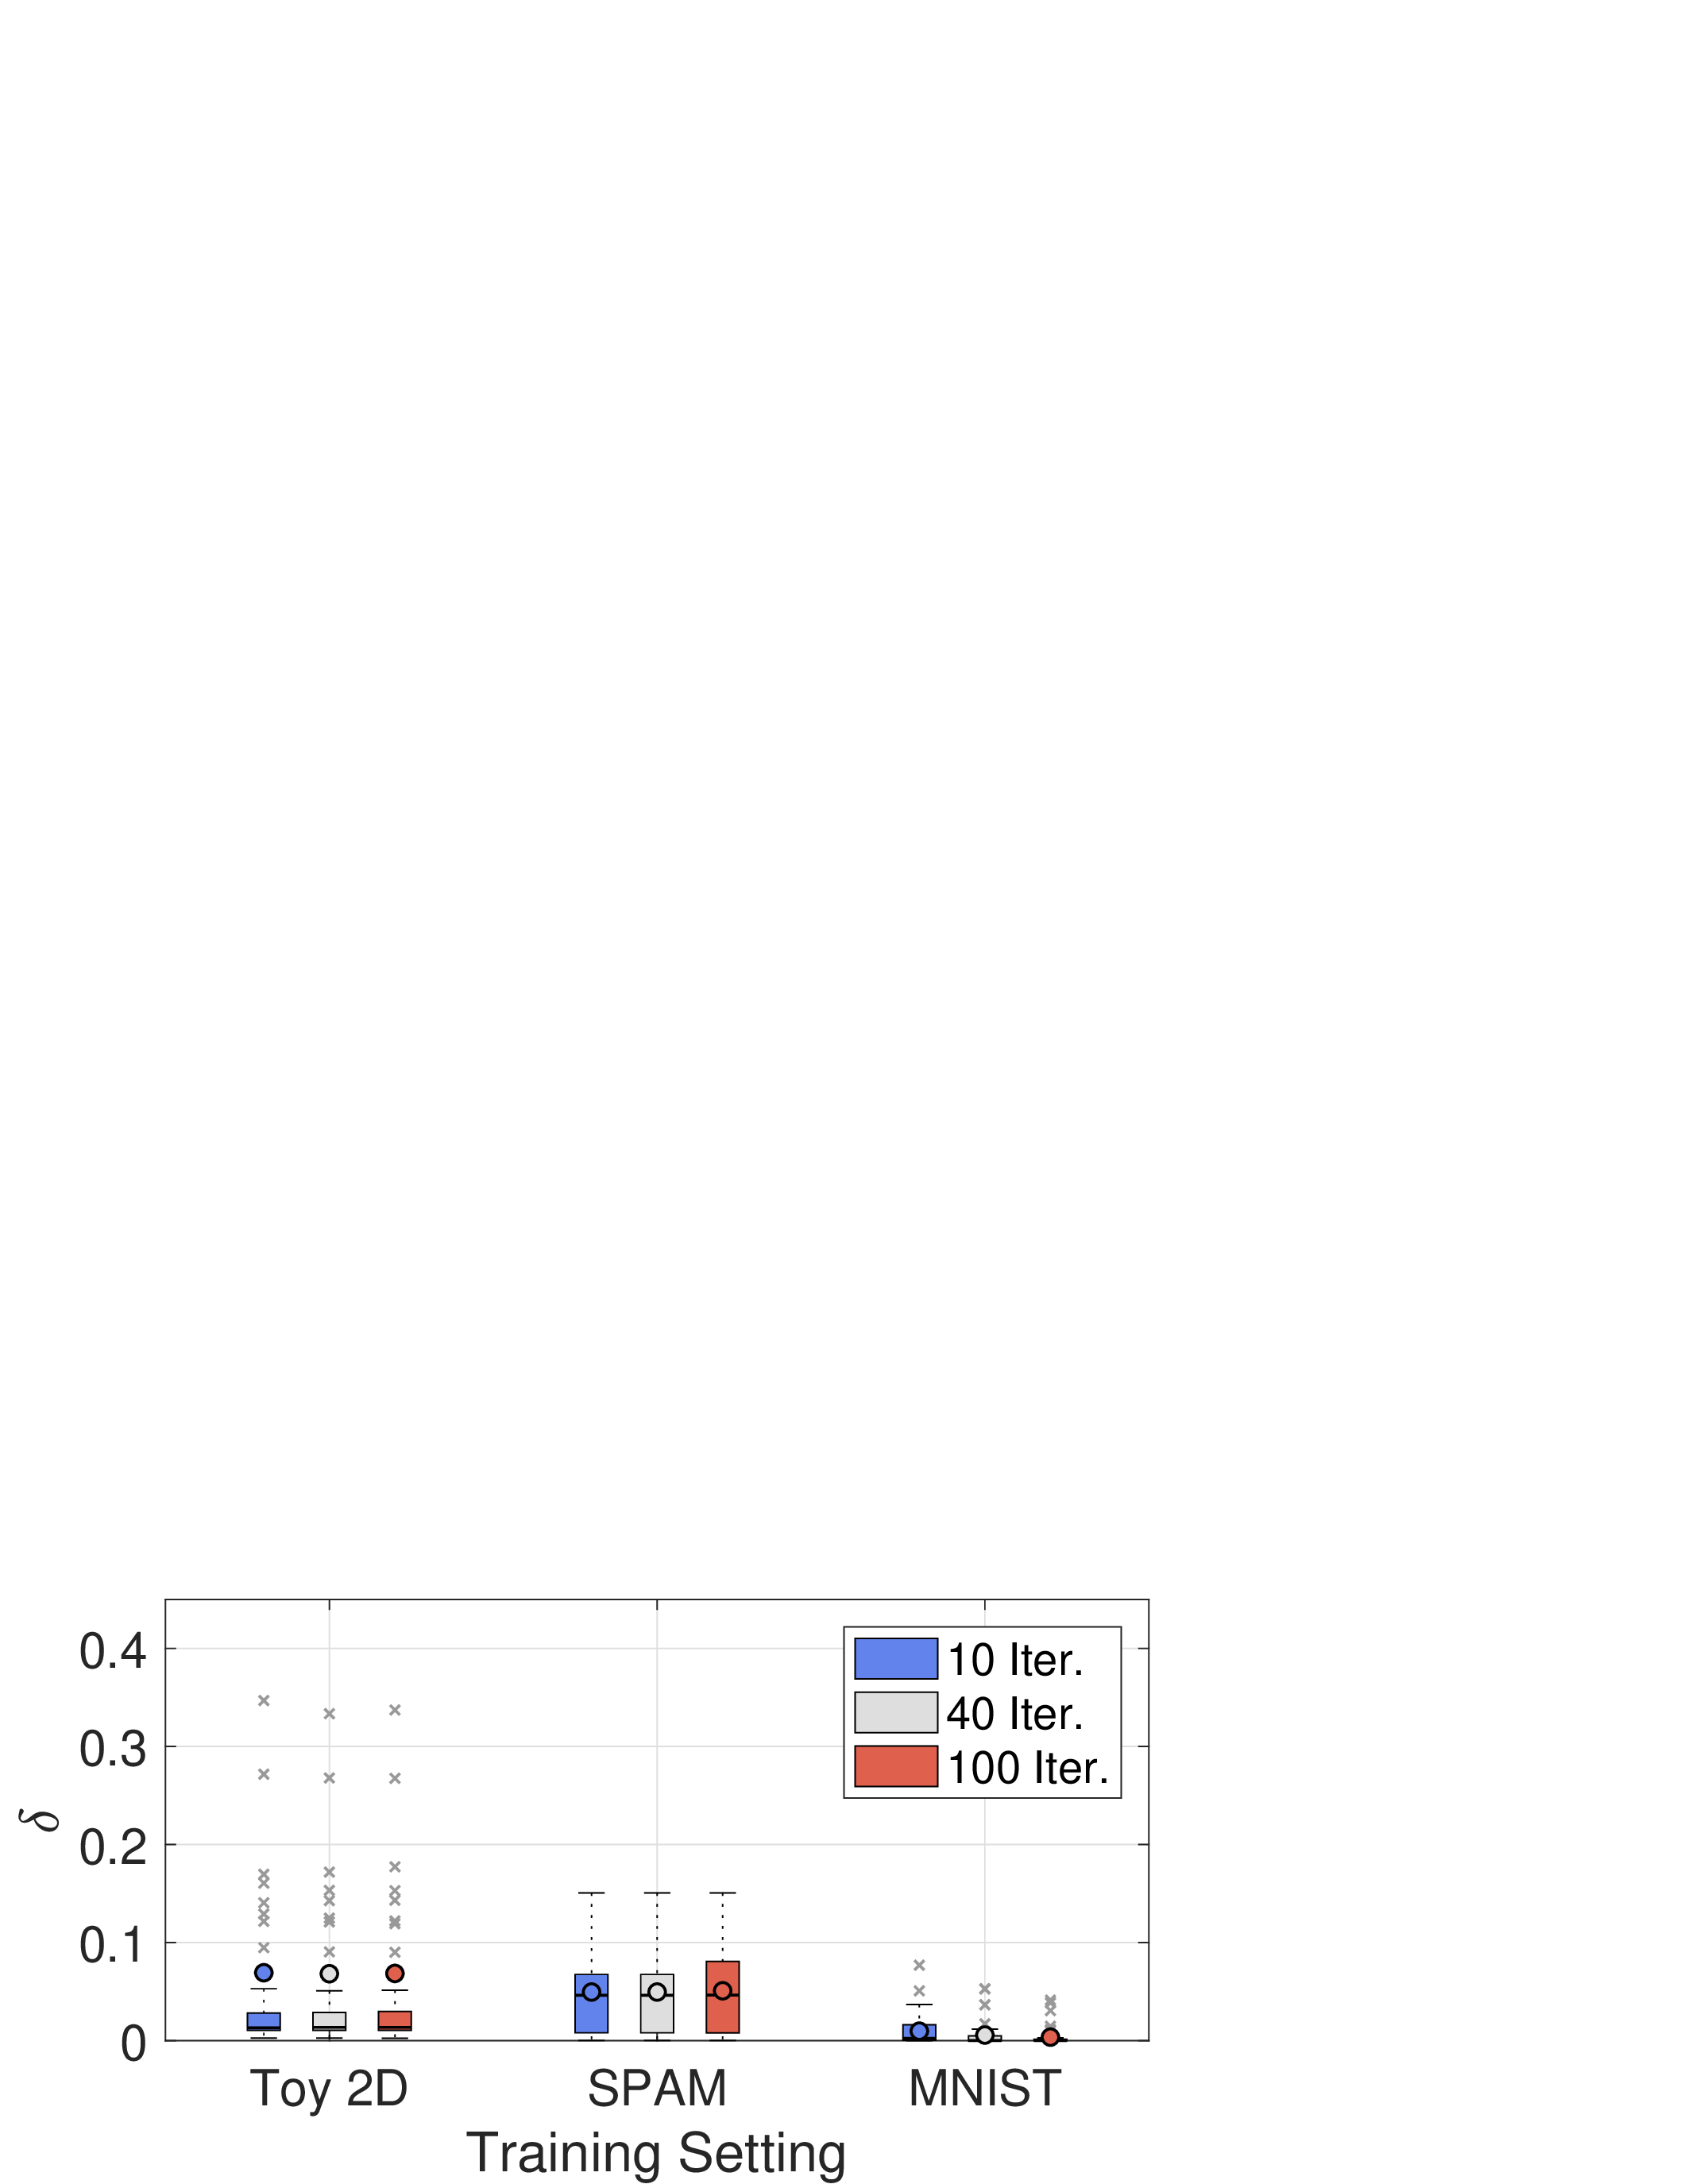}

    %%: SUGGESTED NEW VERSION:
      %%IMPORTANT: IF YOU USE THIS NEW VERSION, ALSO COMMENT OUT LAST 2 LINES OF CAPTION ABOUT LEFT AND RIGHT COLUMN
    
	\includegraphics[width = 0.32\textwidth]{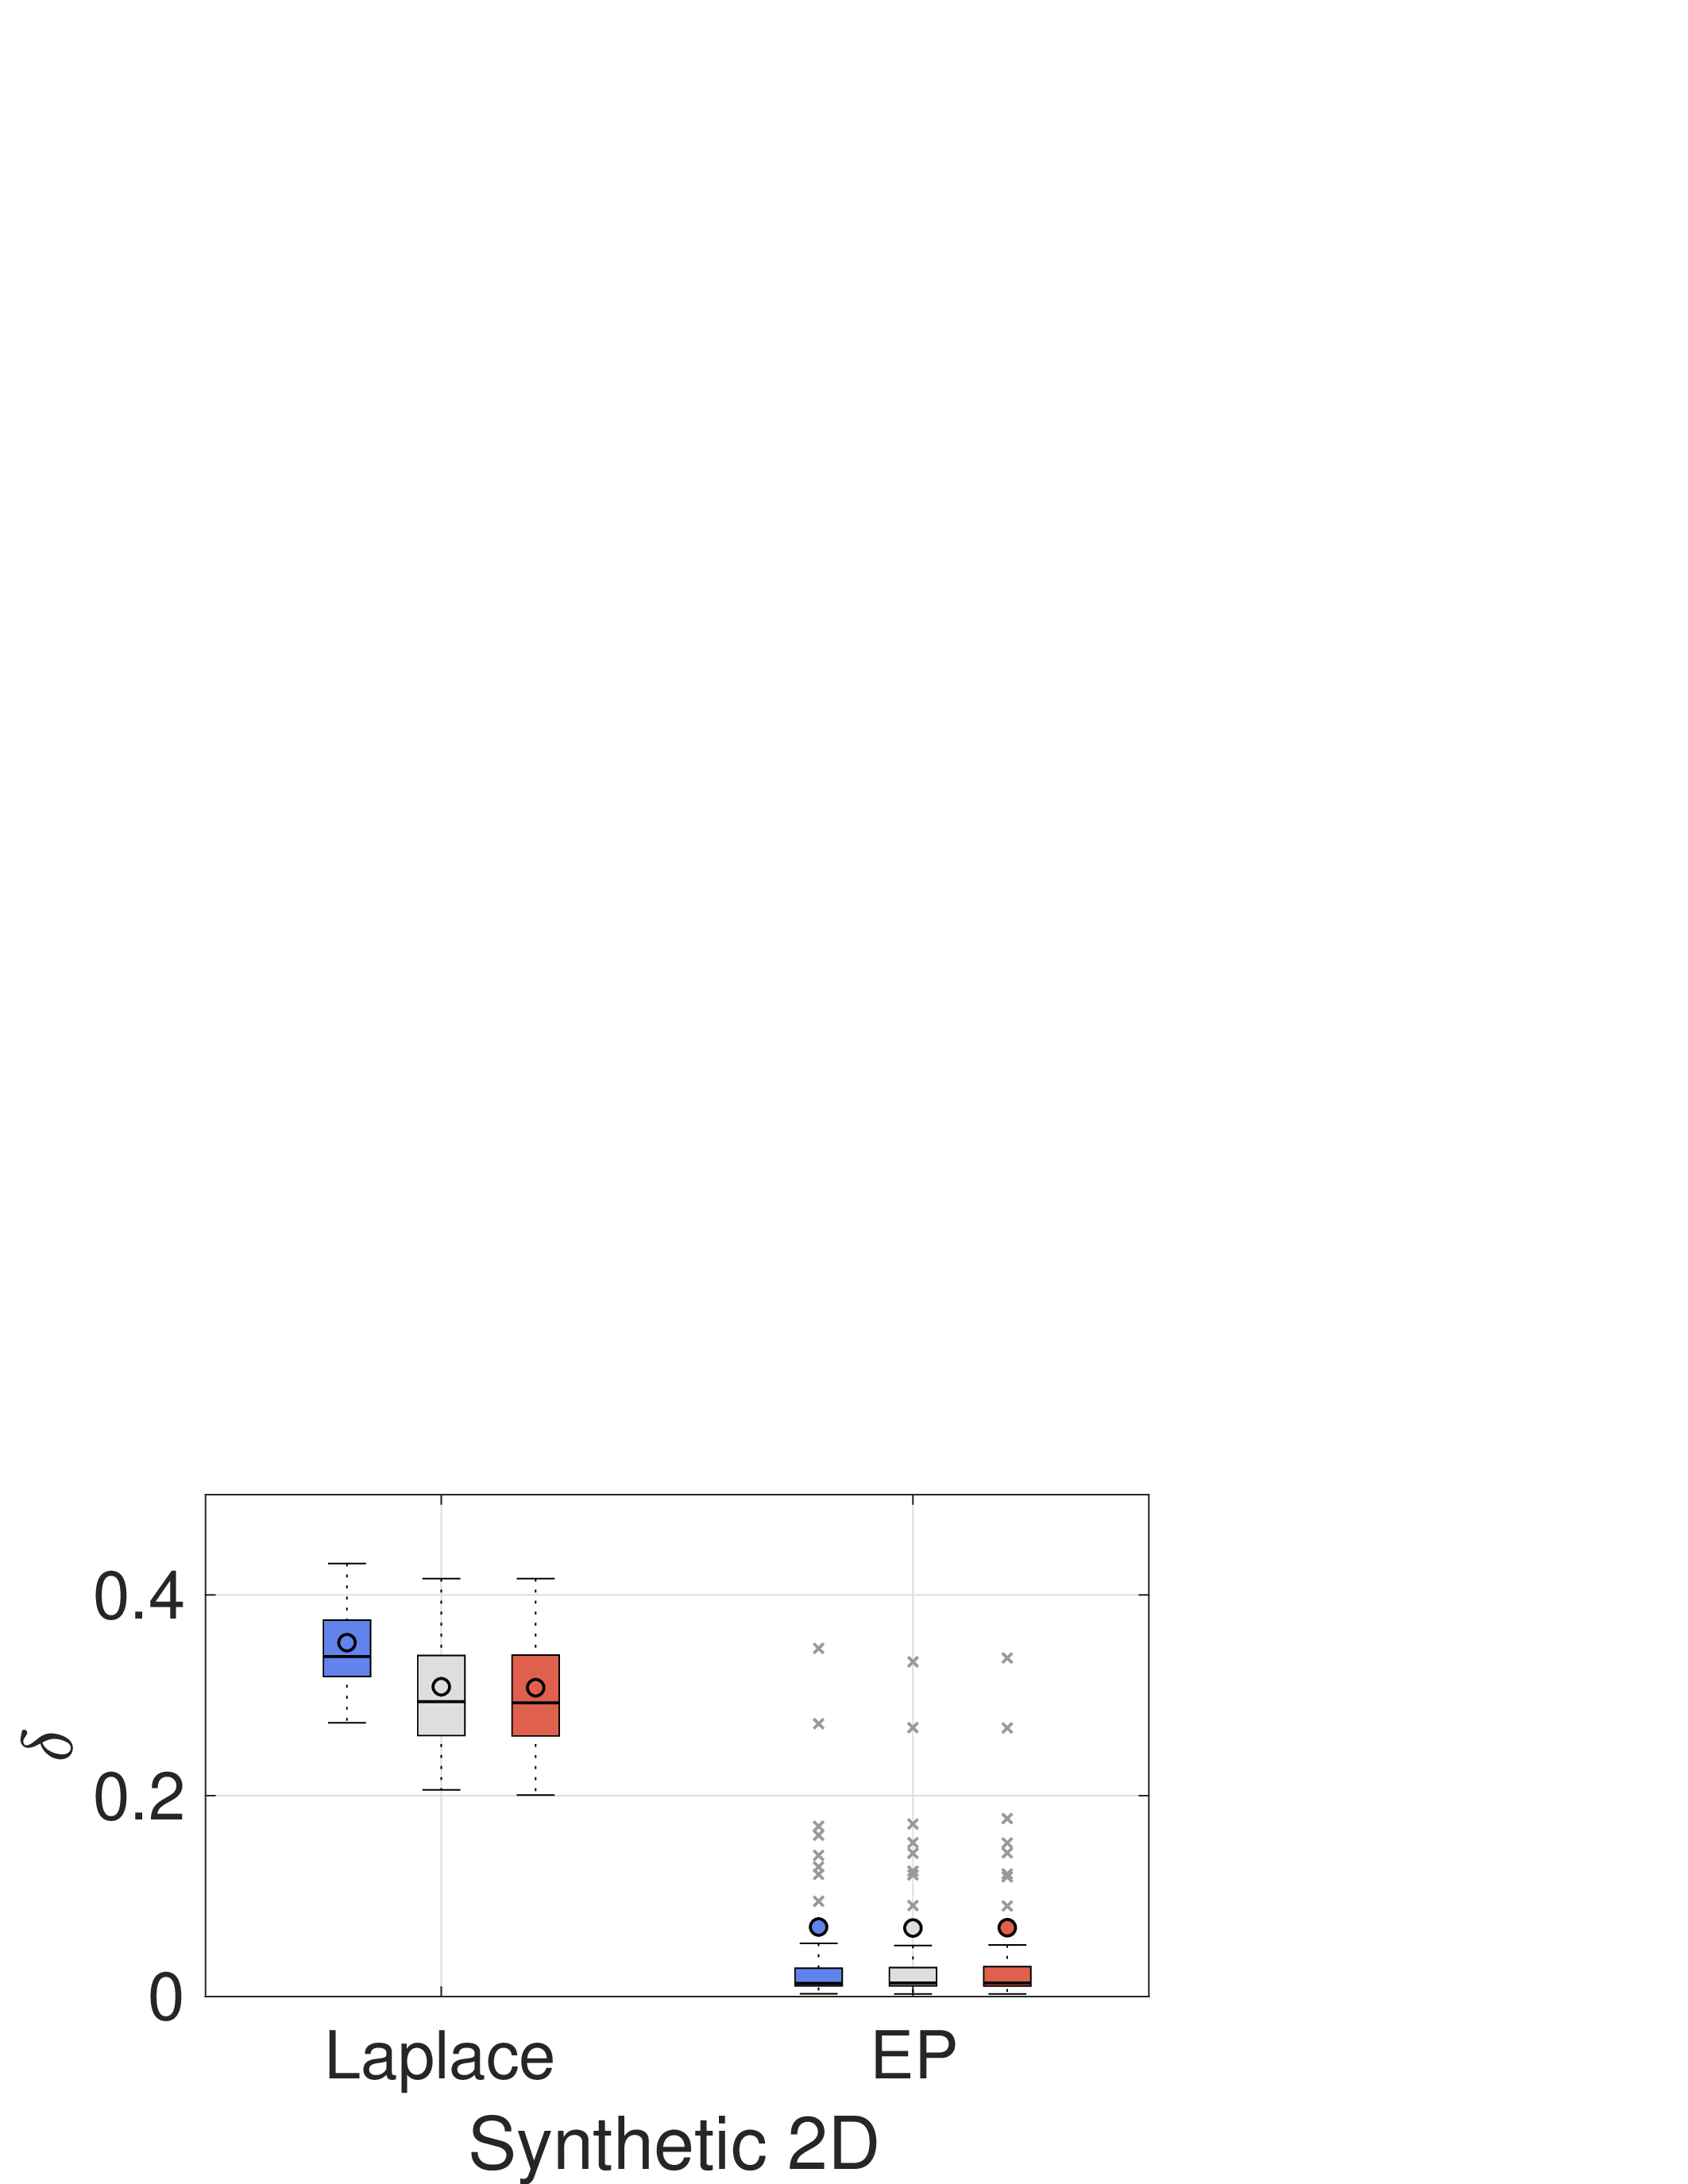}
	\includegraphics[ width = 0.32\textwidth]{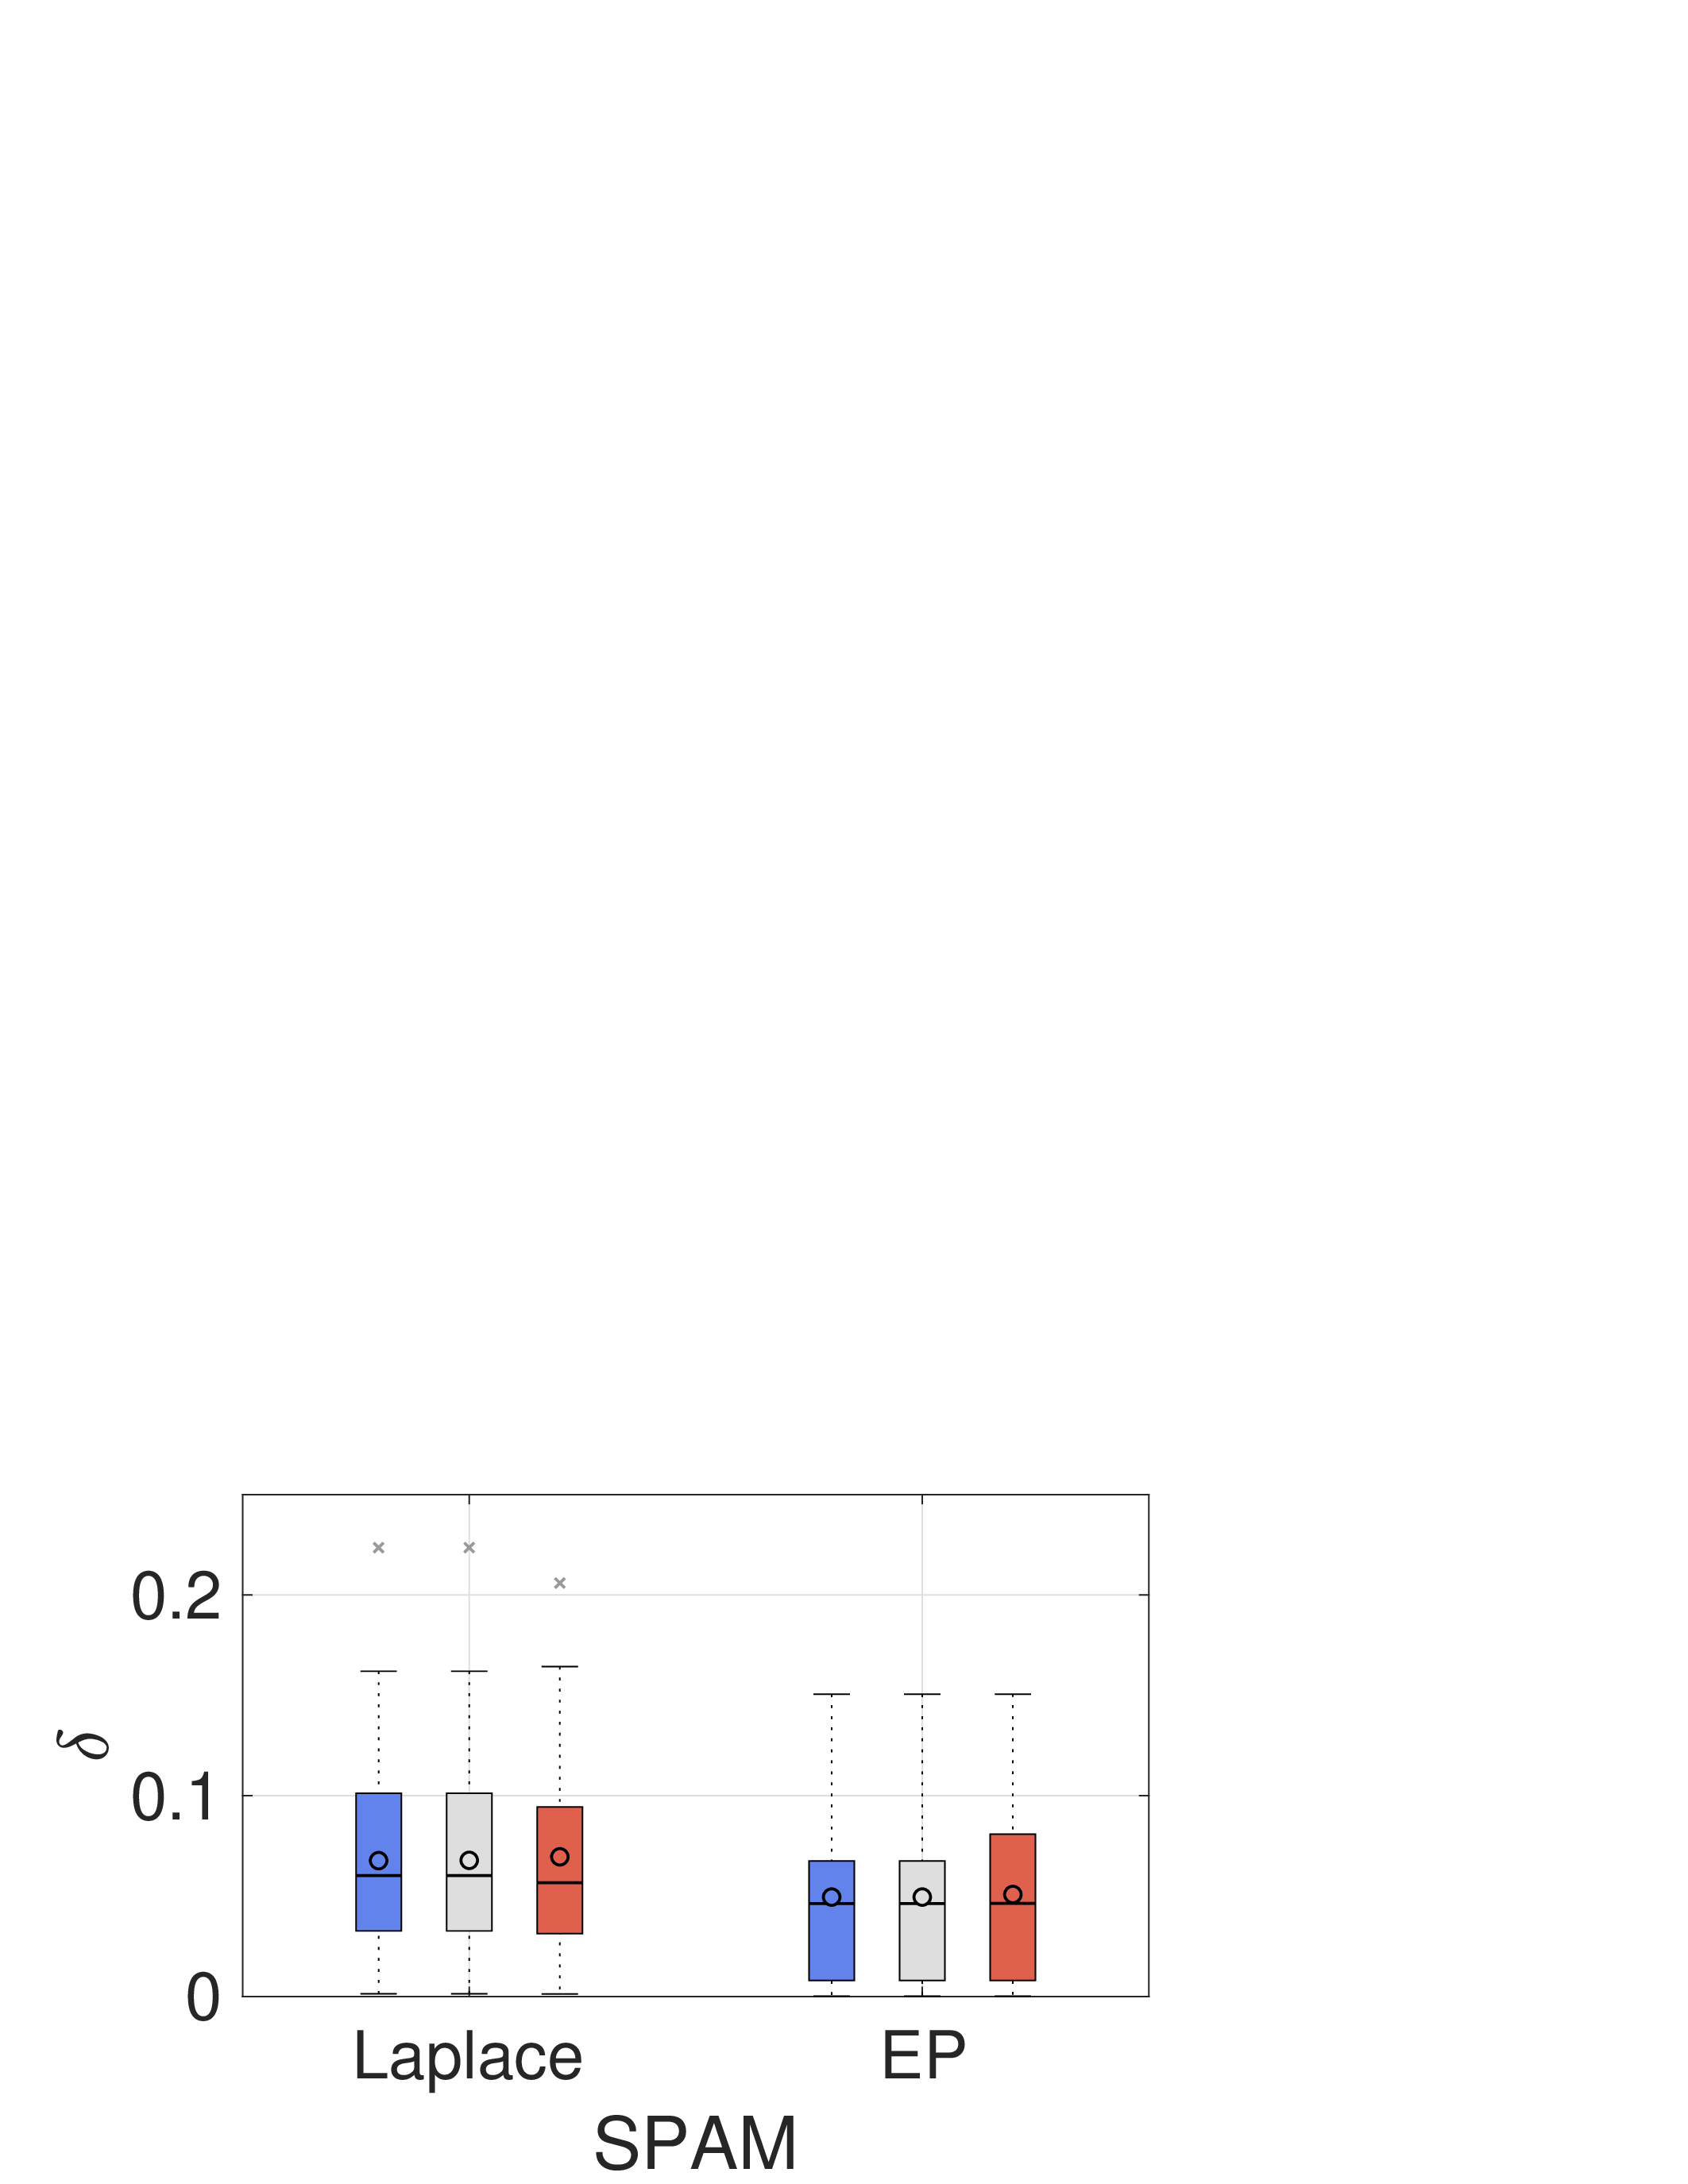}
	\includegraphics[ width = 0.32\textwidth]{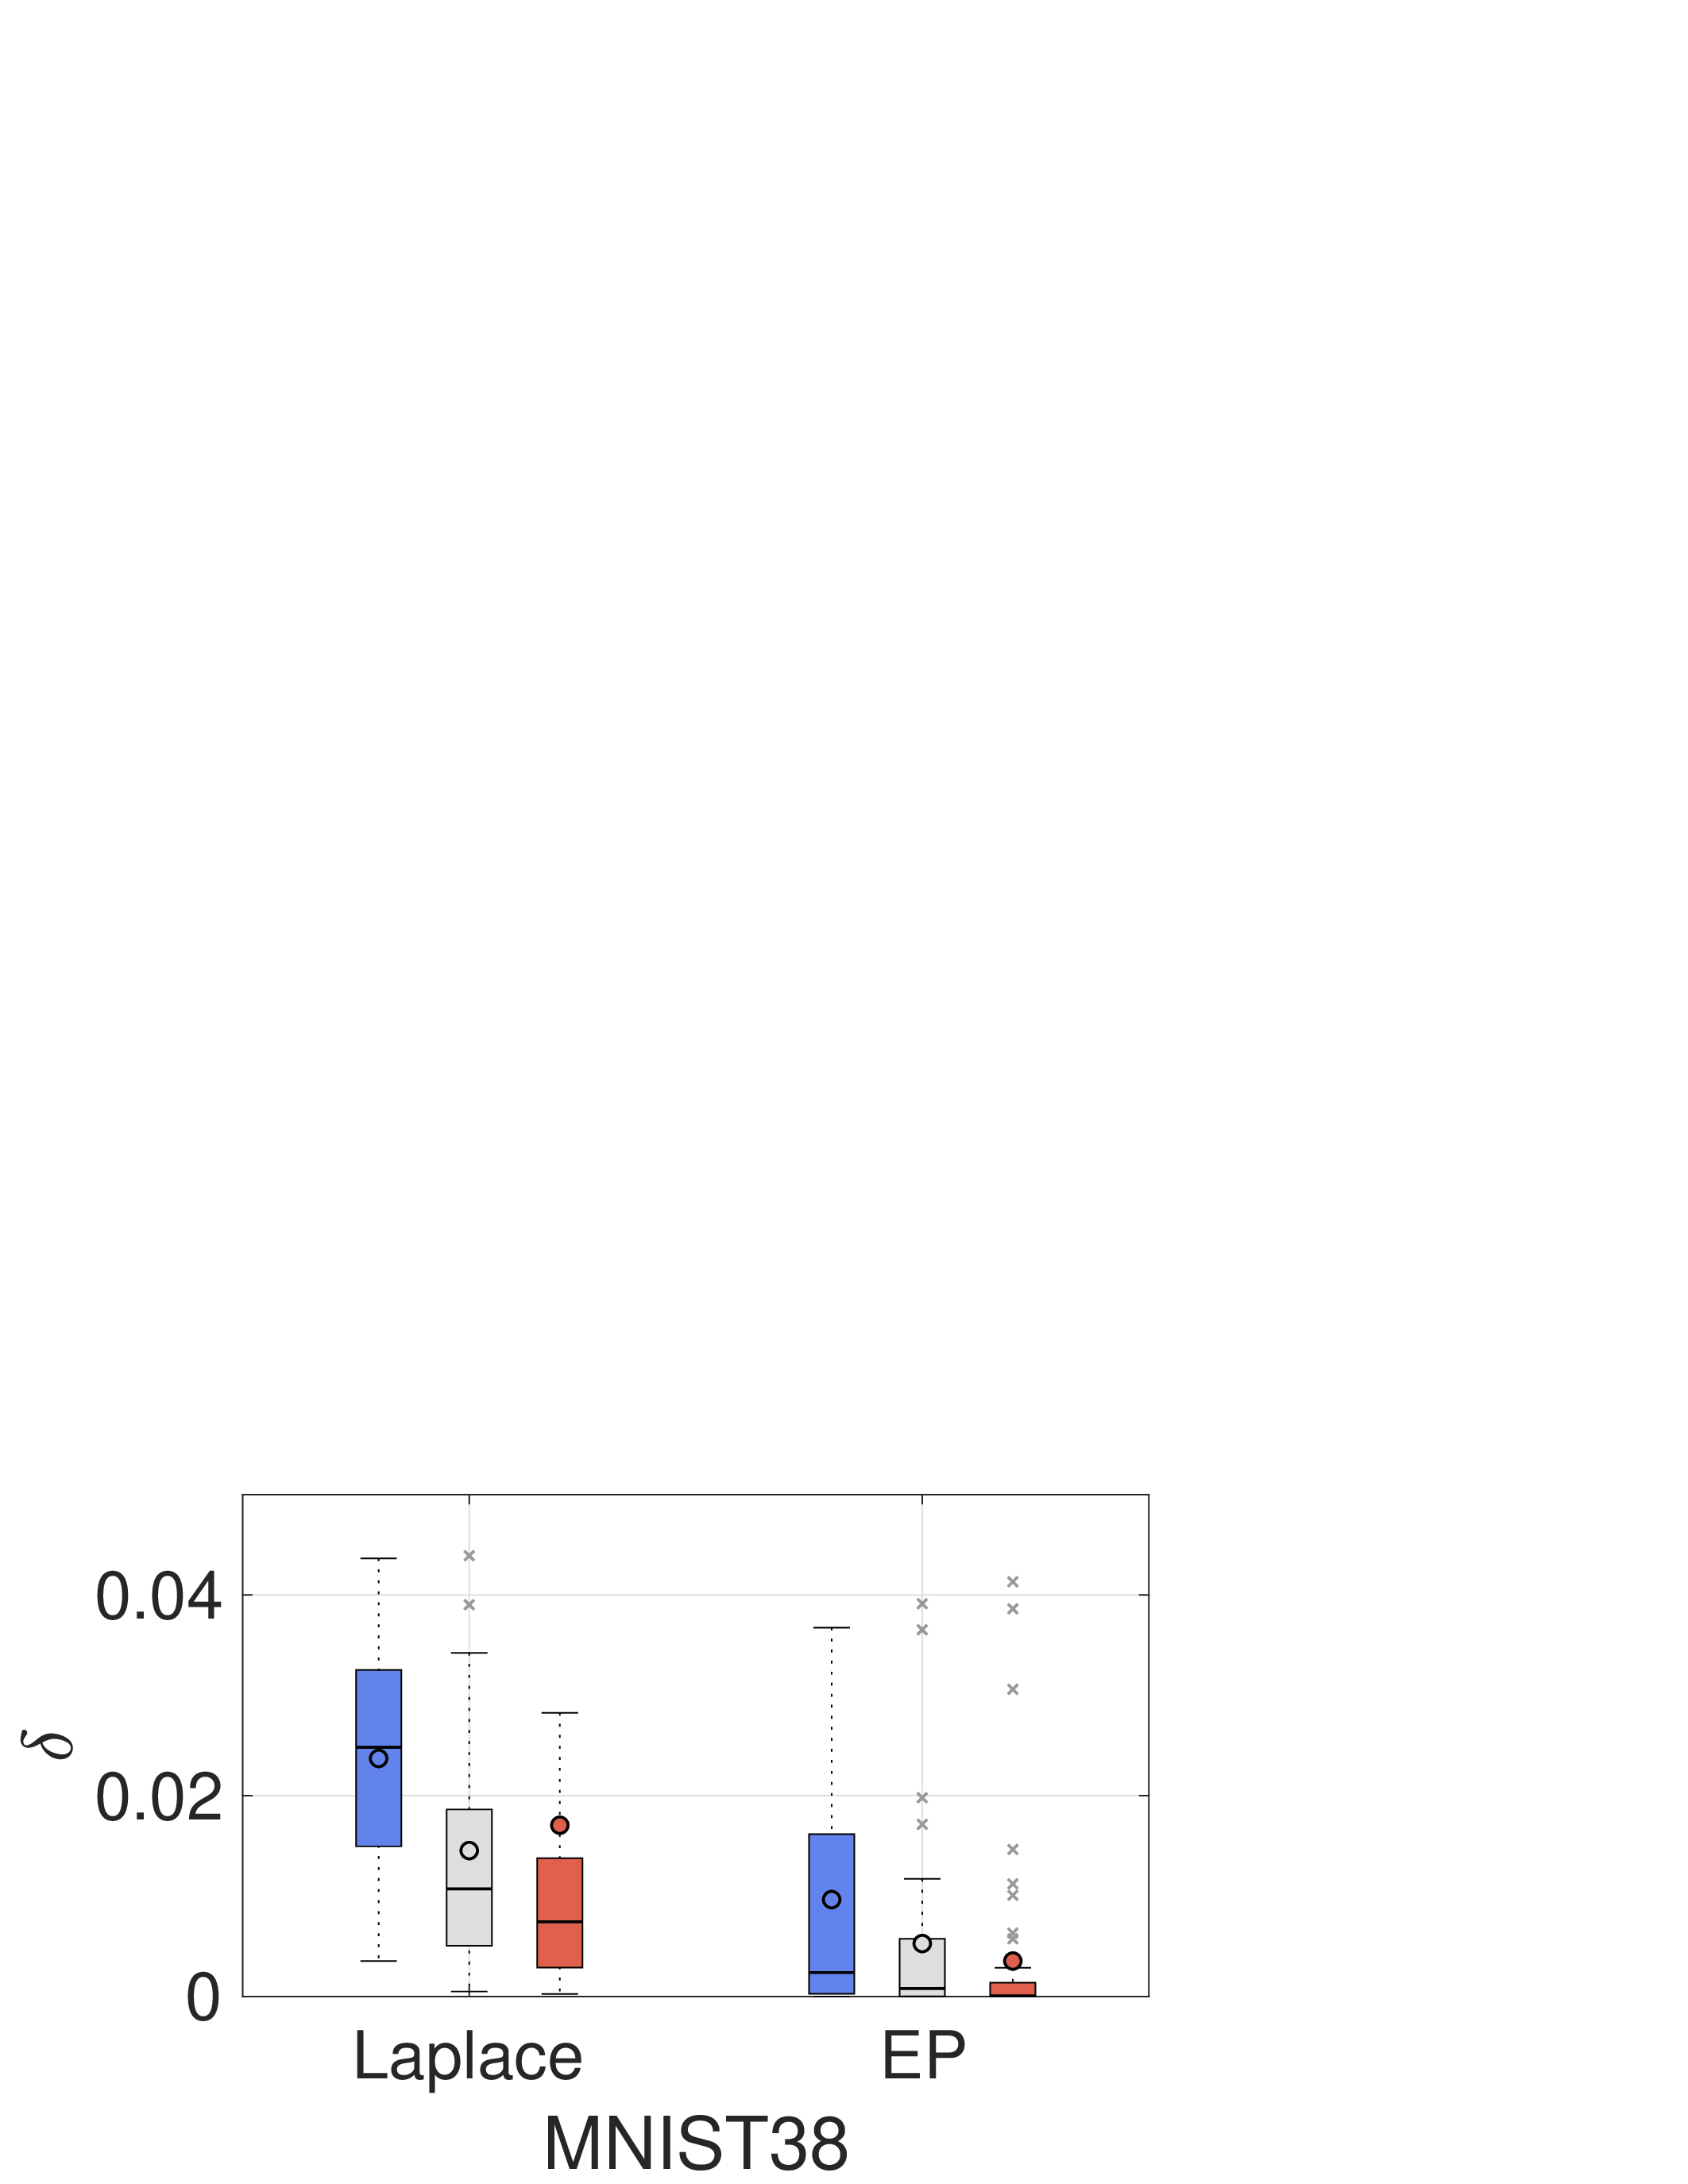}
	{\hspace*{0.2cm}  \includegraphics[width = 0.45\textwidth]{figures/LegendRobustness2.pdf}} 
	
	%\caption{Boxplots for empirical distribution (i.e.\ wrt to the test set) of robustness on the three dataset considered in this paper, comparing Lapalace and EP approximation. \textbf{Left plot}: Kernel parameters estimated using 10 optimization iterations.  \textbf{Right plot}:  Kernel parameters estimated using 100 optimization iterations.}
	\caption{Boxplots for empirical distribution (i.e.\ wrt to the test set) of robustness on the three datasets considered in this paper, comparing Lapalace and EP approximation (a smaller $\delta$ implies a more robust model). 
	%\textbf{Left plot}: Laplace posterior approximation.  \textbf{Right plot}: EP posterior approximation.
	}
	%\label{fig:Robustness}
\end{figure}

and possible new figure for Interpretability in Section 6.3:

\label{subsec:interpretability}
\begin{wrapfigure}{r}{0.5\textwidth}
  	\centering
	\includegraphics[clip = on, trim = 10mm 10mm 10mm 10mm ,width = 0.15\textwidth]{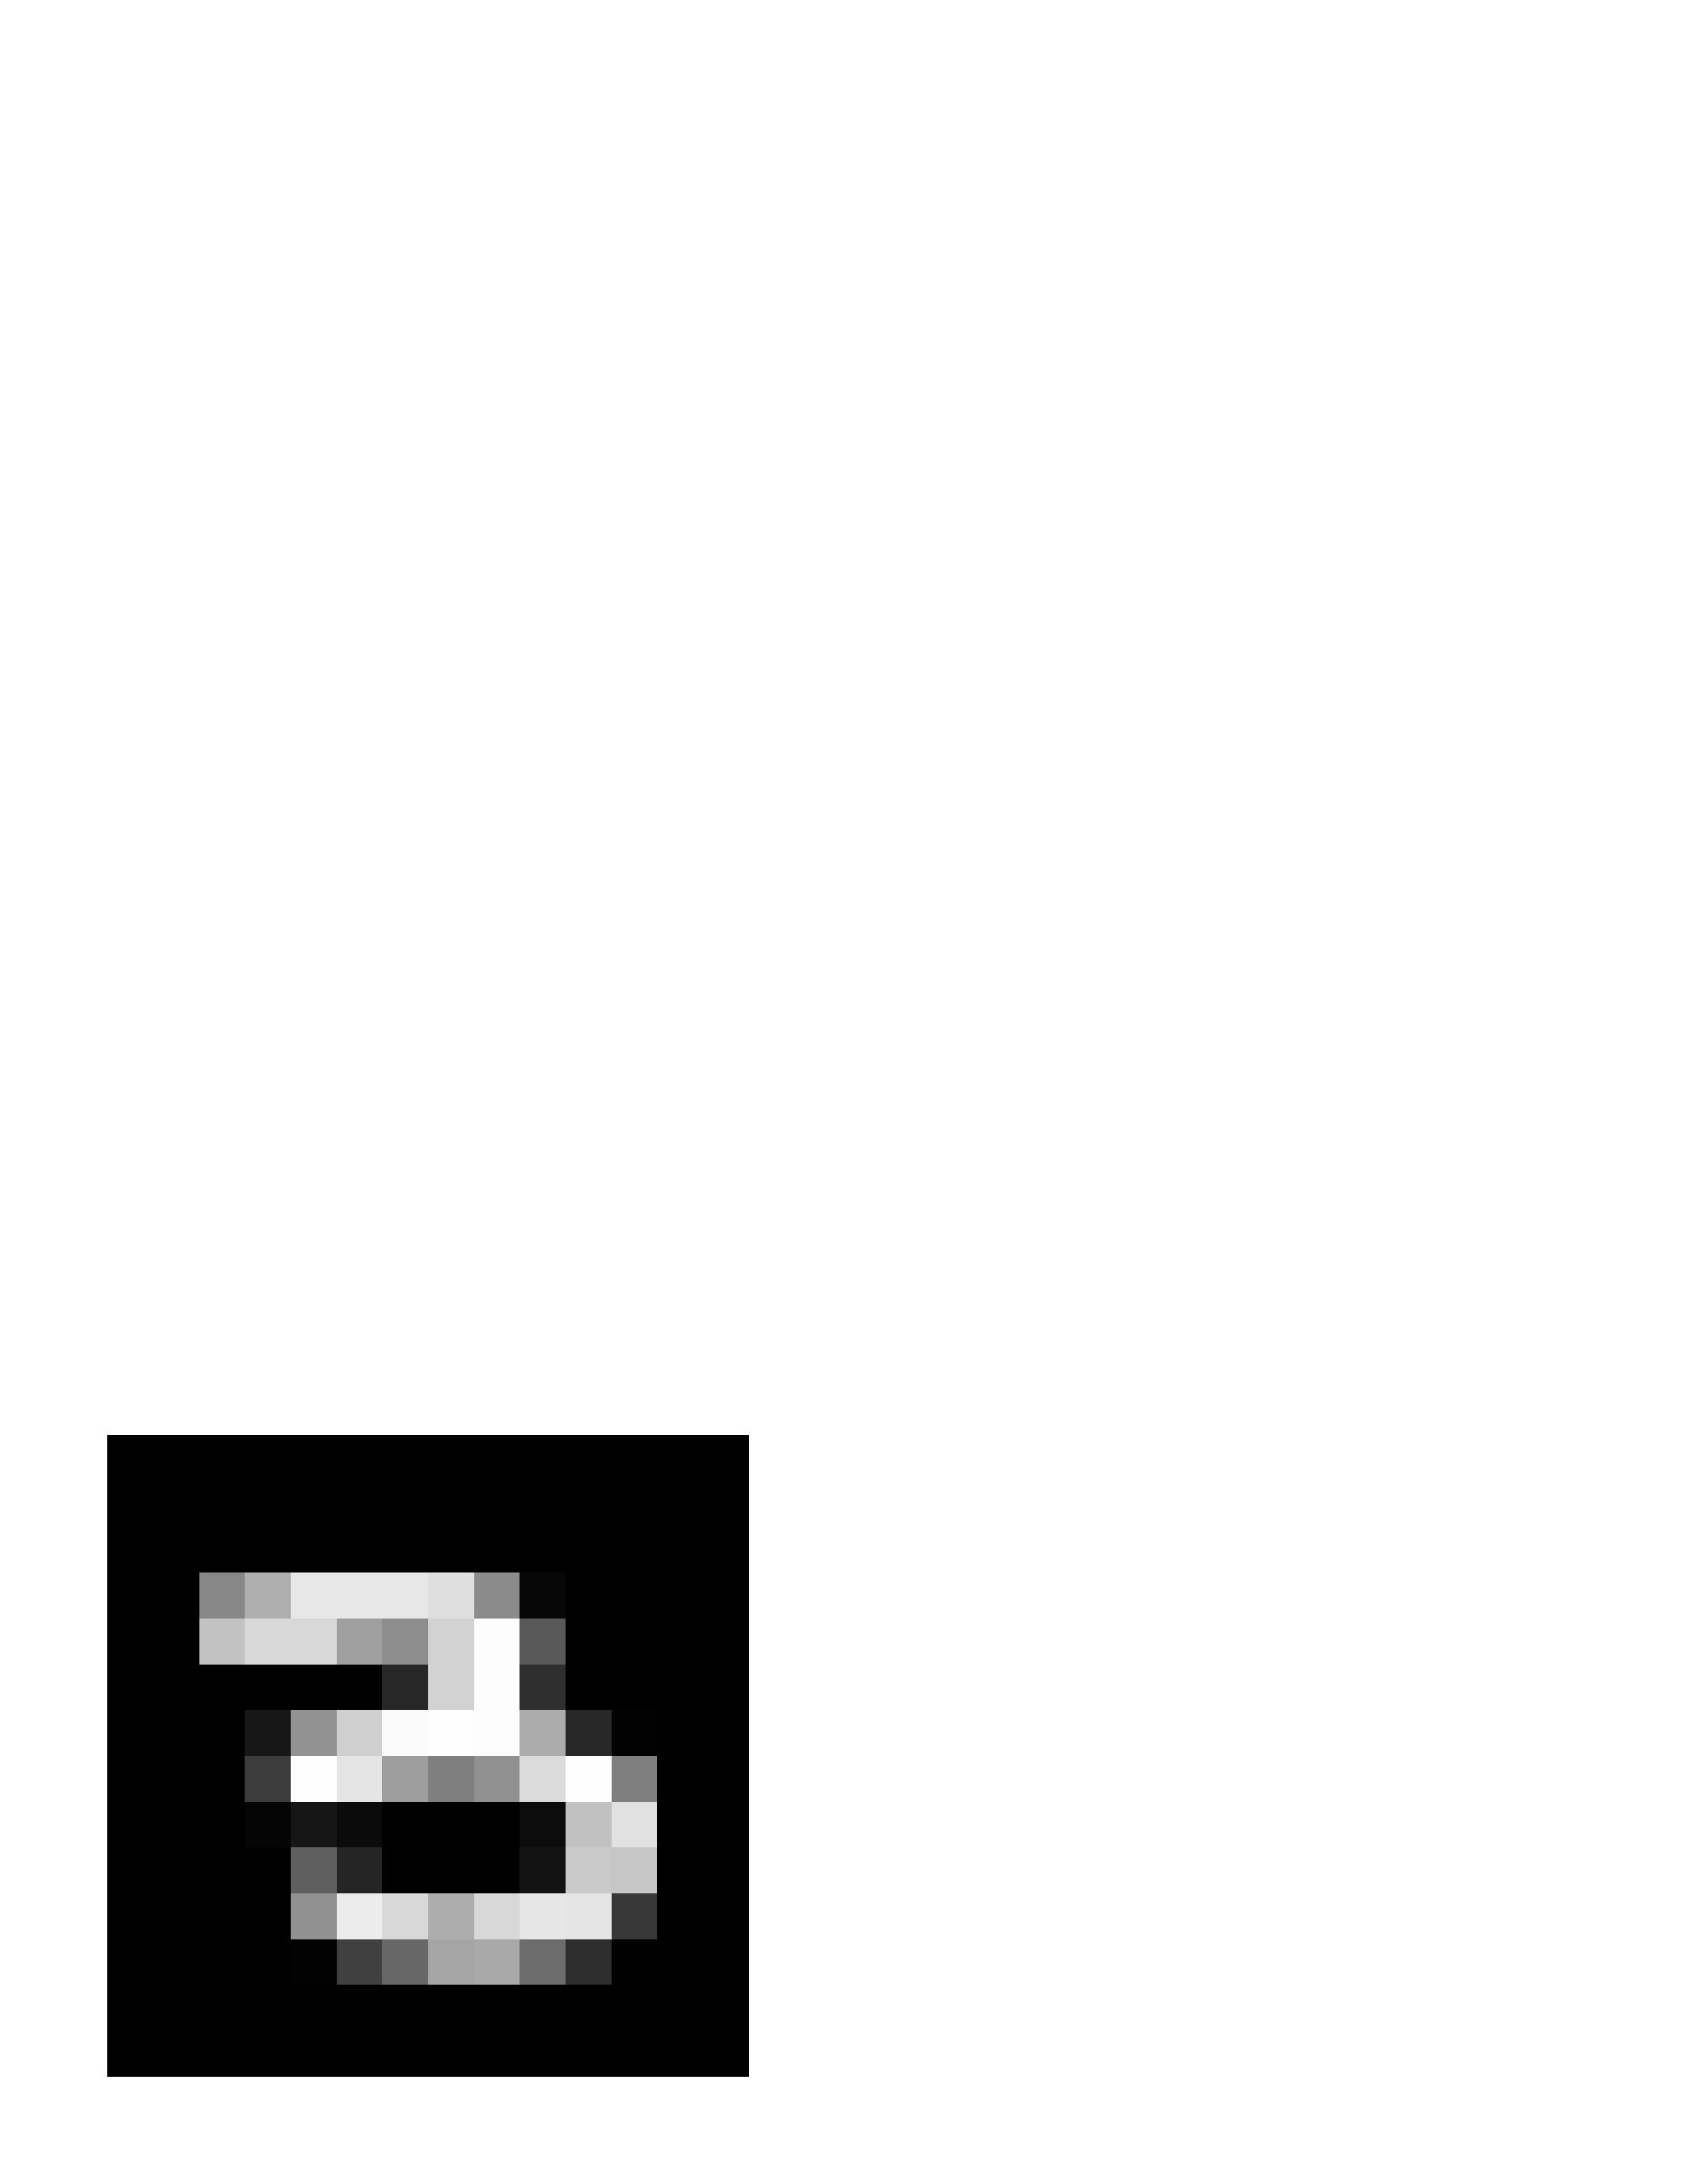}
	\includegraphics[clip = on, trim = 10mm 10mm 10mm 10mm ,width = 0.15\textwidth]{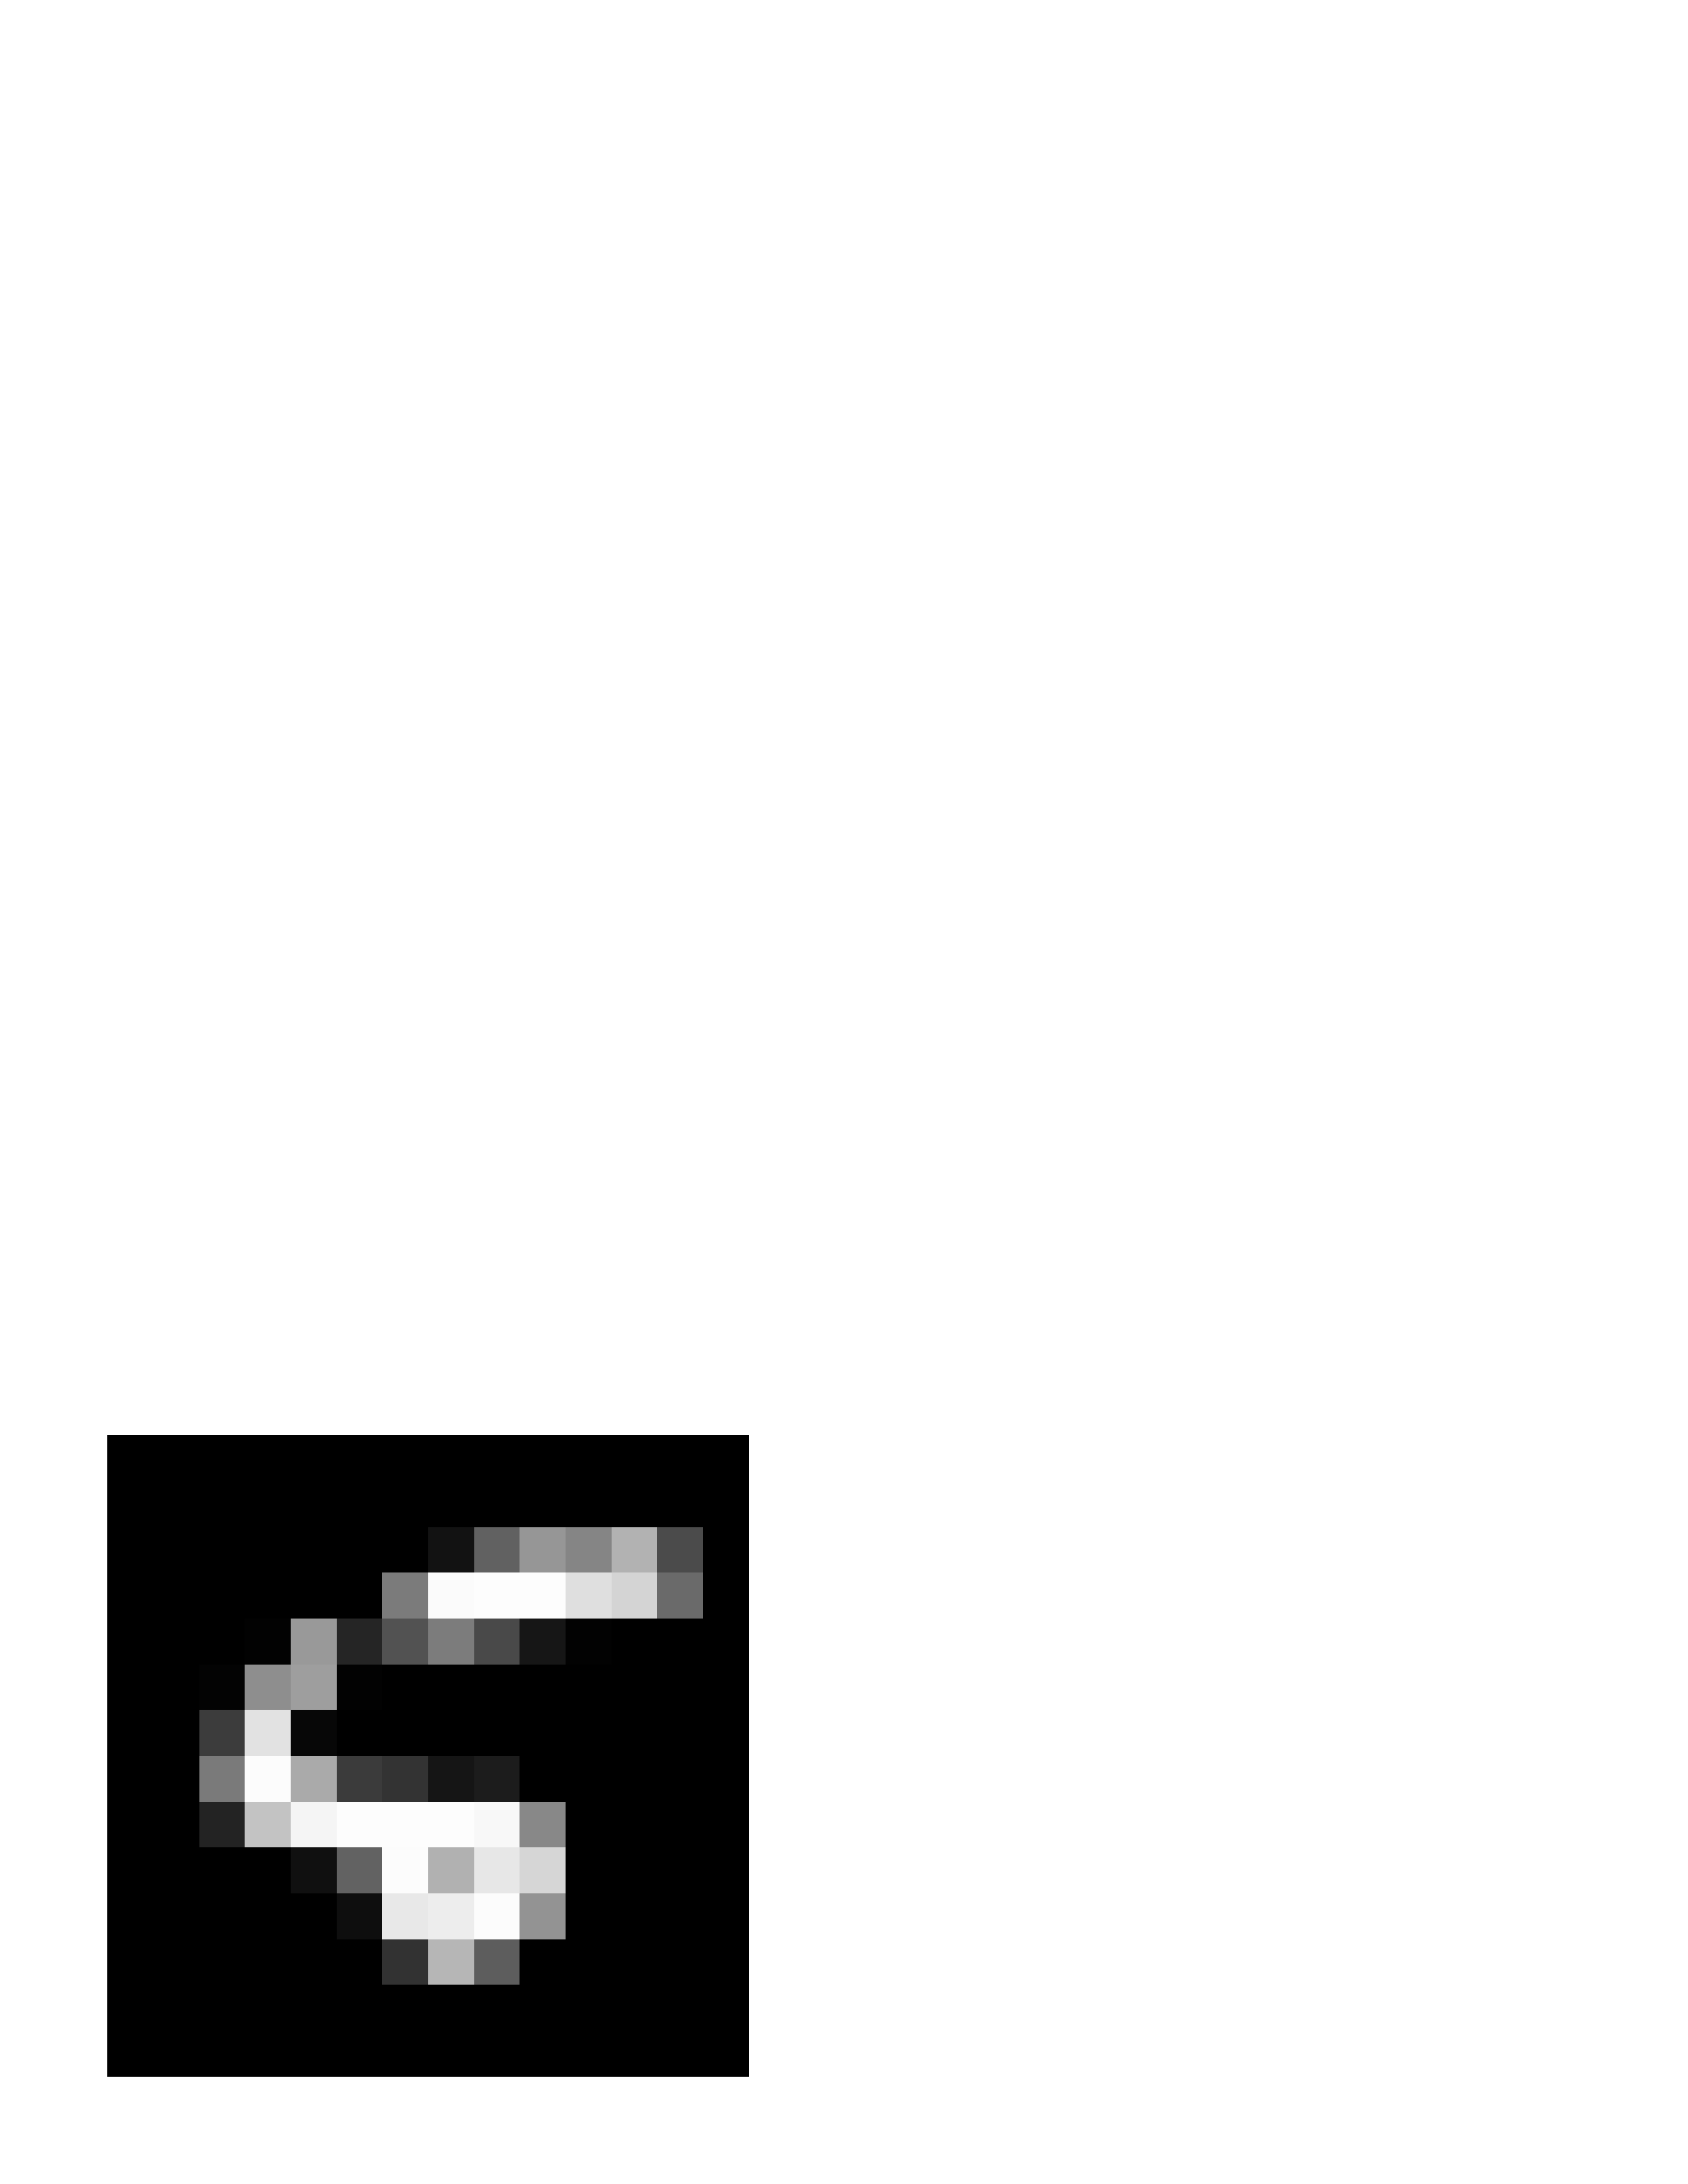}
	\includegraphics[clip = on, trim = 10mm 10mm 10mm 10mm ,width = 0.15\textwidth]{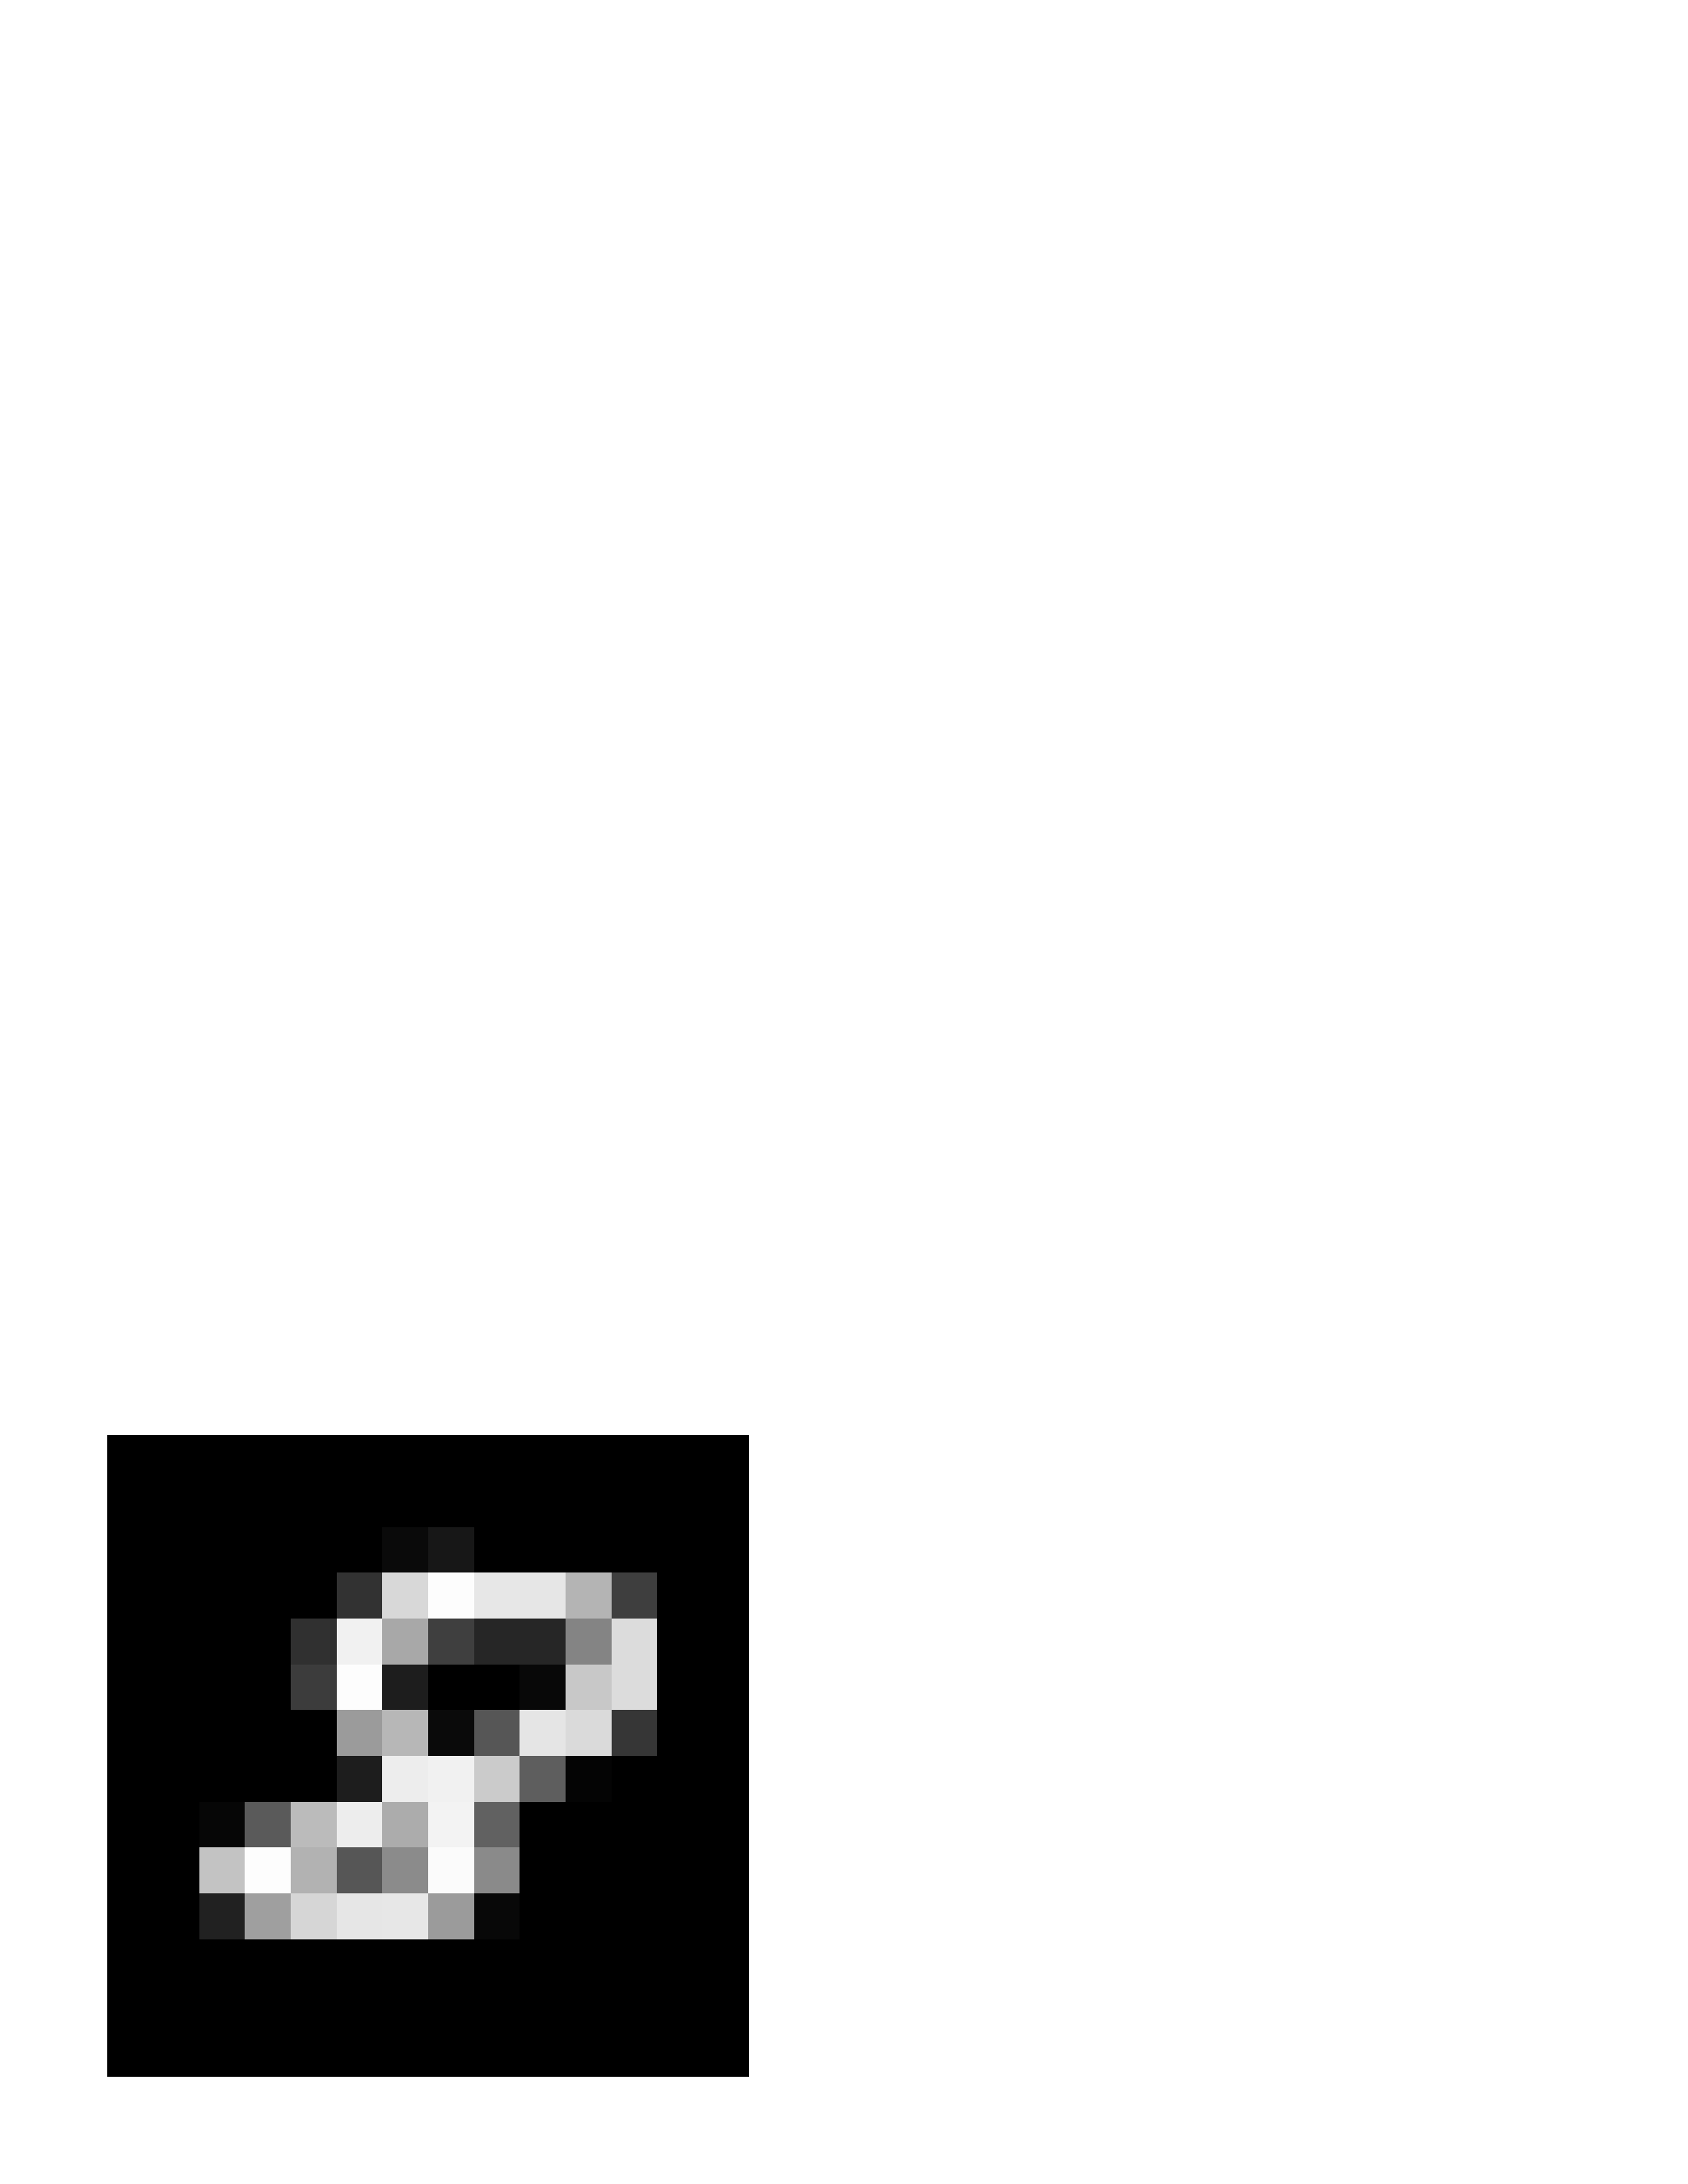} \\ 
	
	\includegraphics[clip = on, trim = 10mm 10mm 10mm 10mm ,width = 0.15\textwidth]{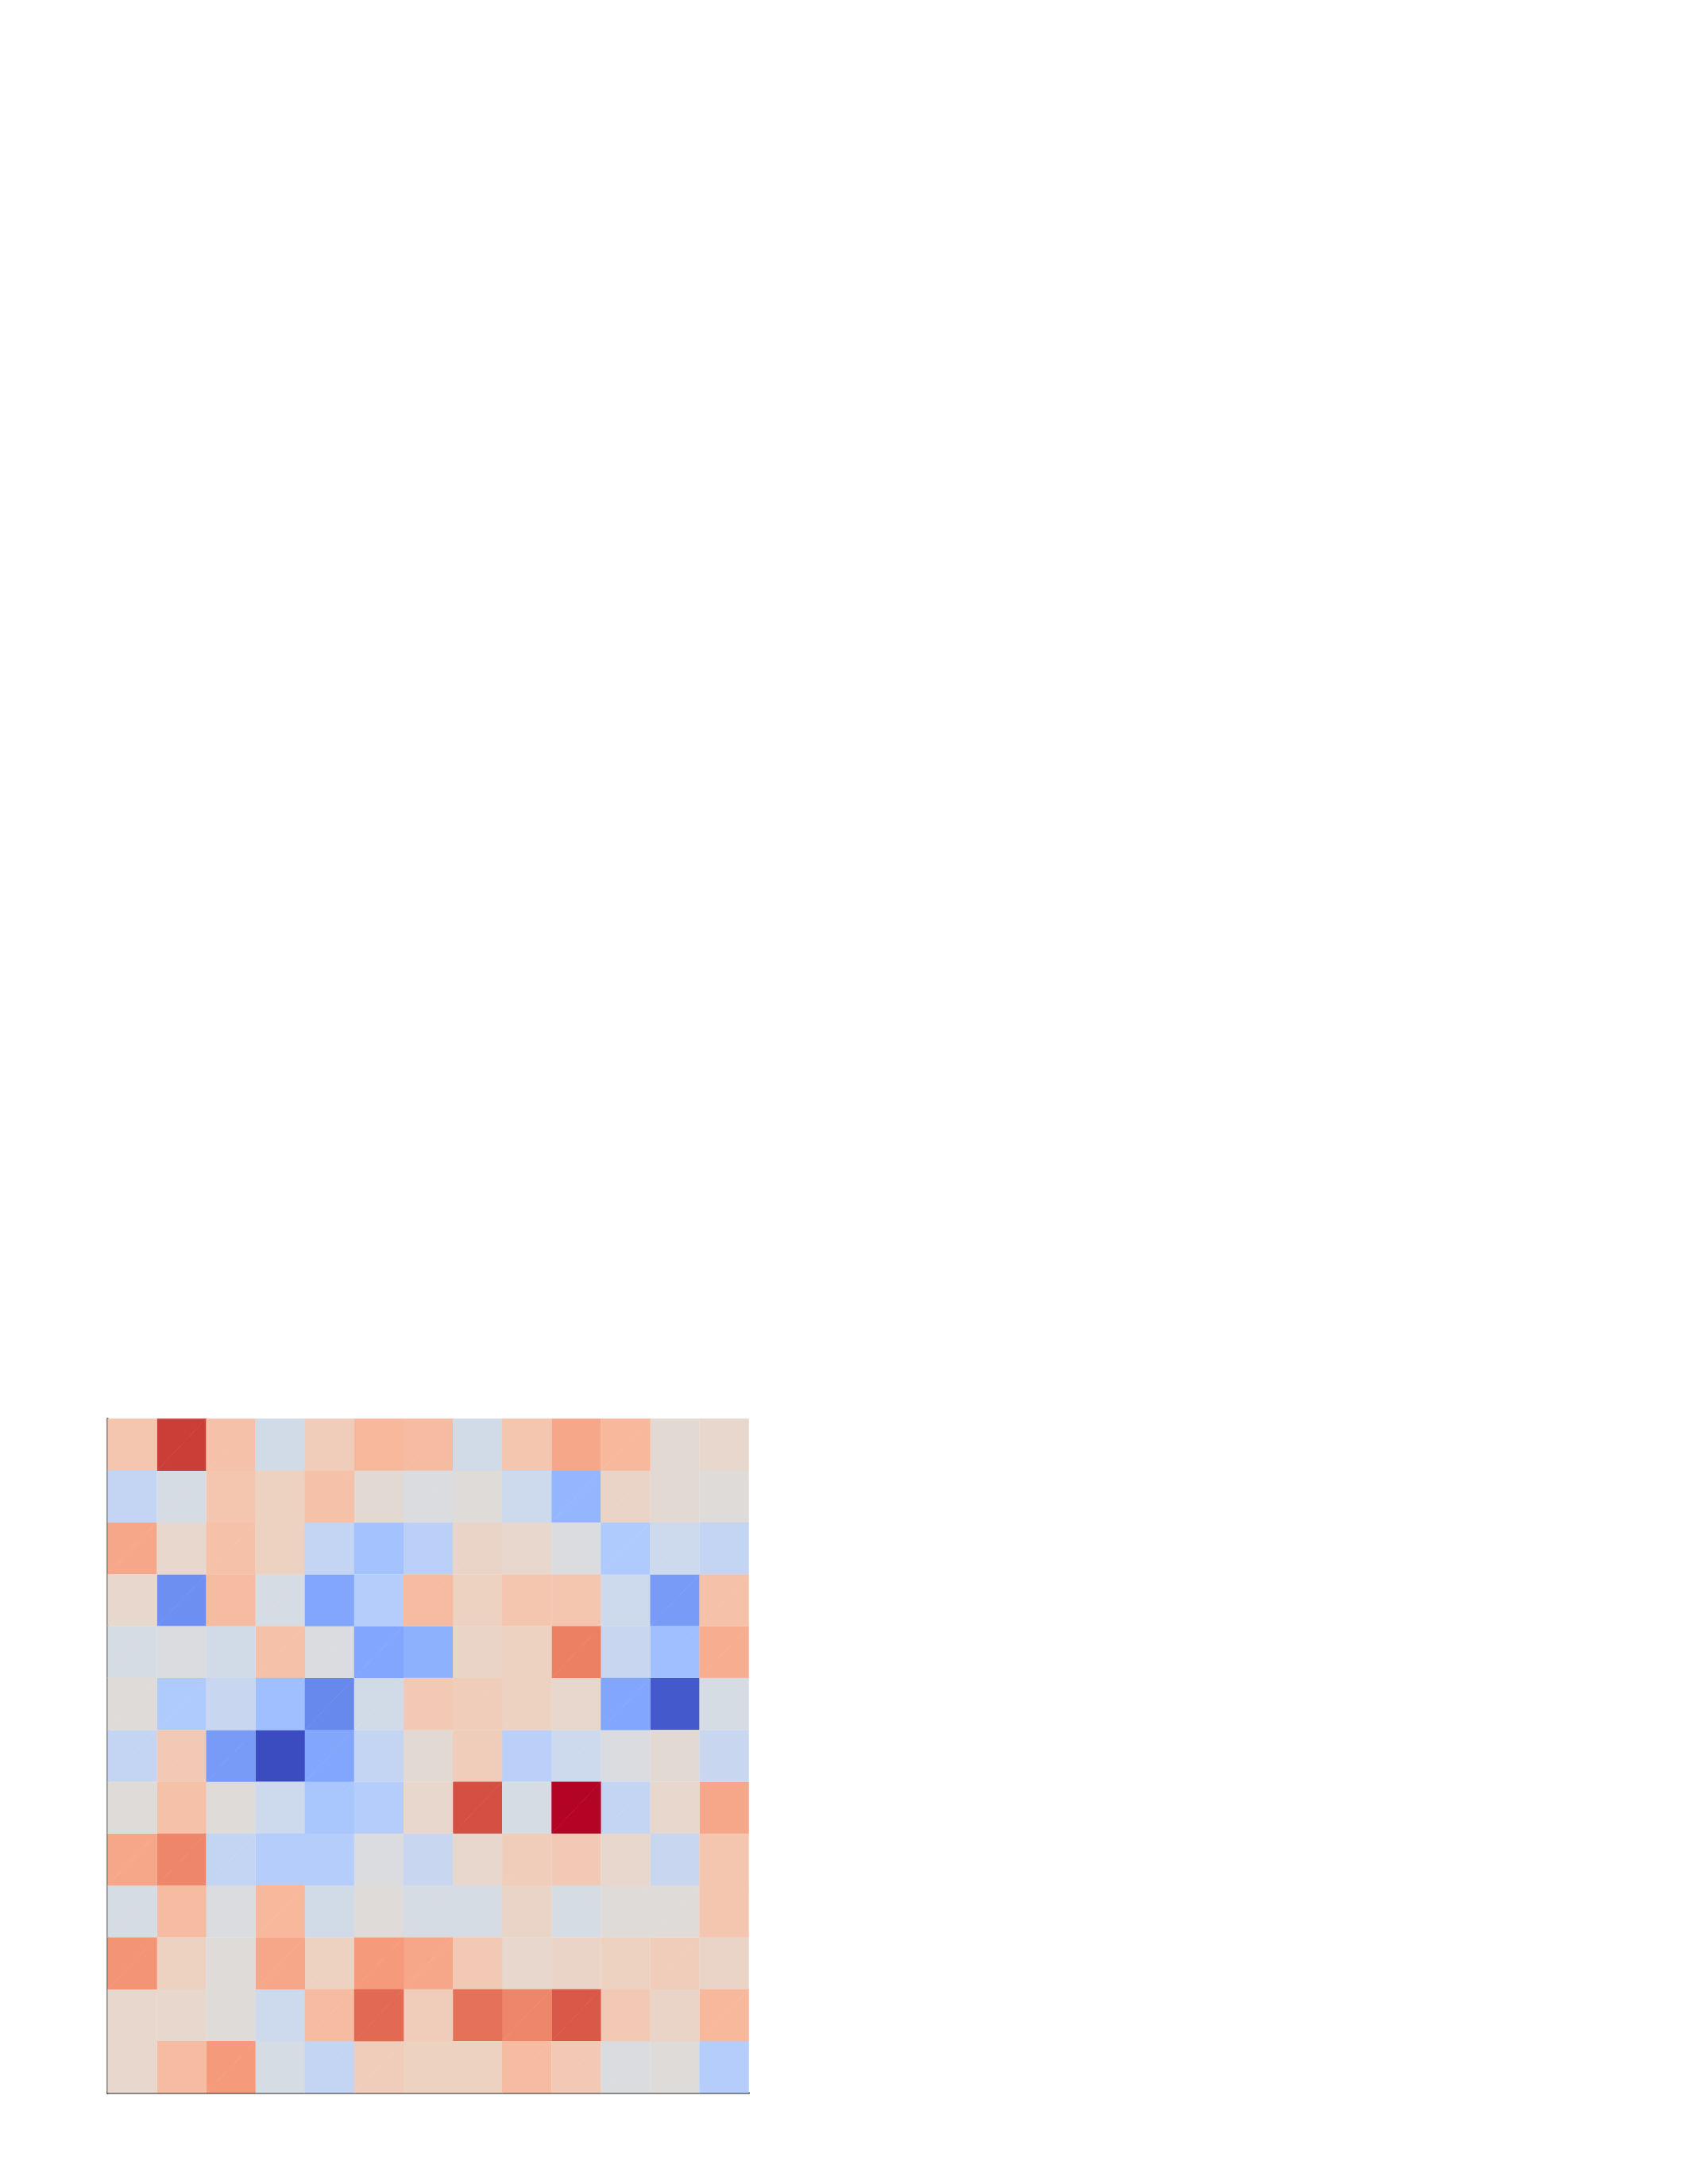}
	\includegraphics[clip = on, trim = 10mm 10mm 10mm 10mm ,width = 0.15\textwidth]{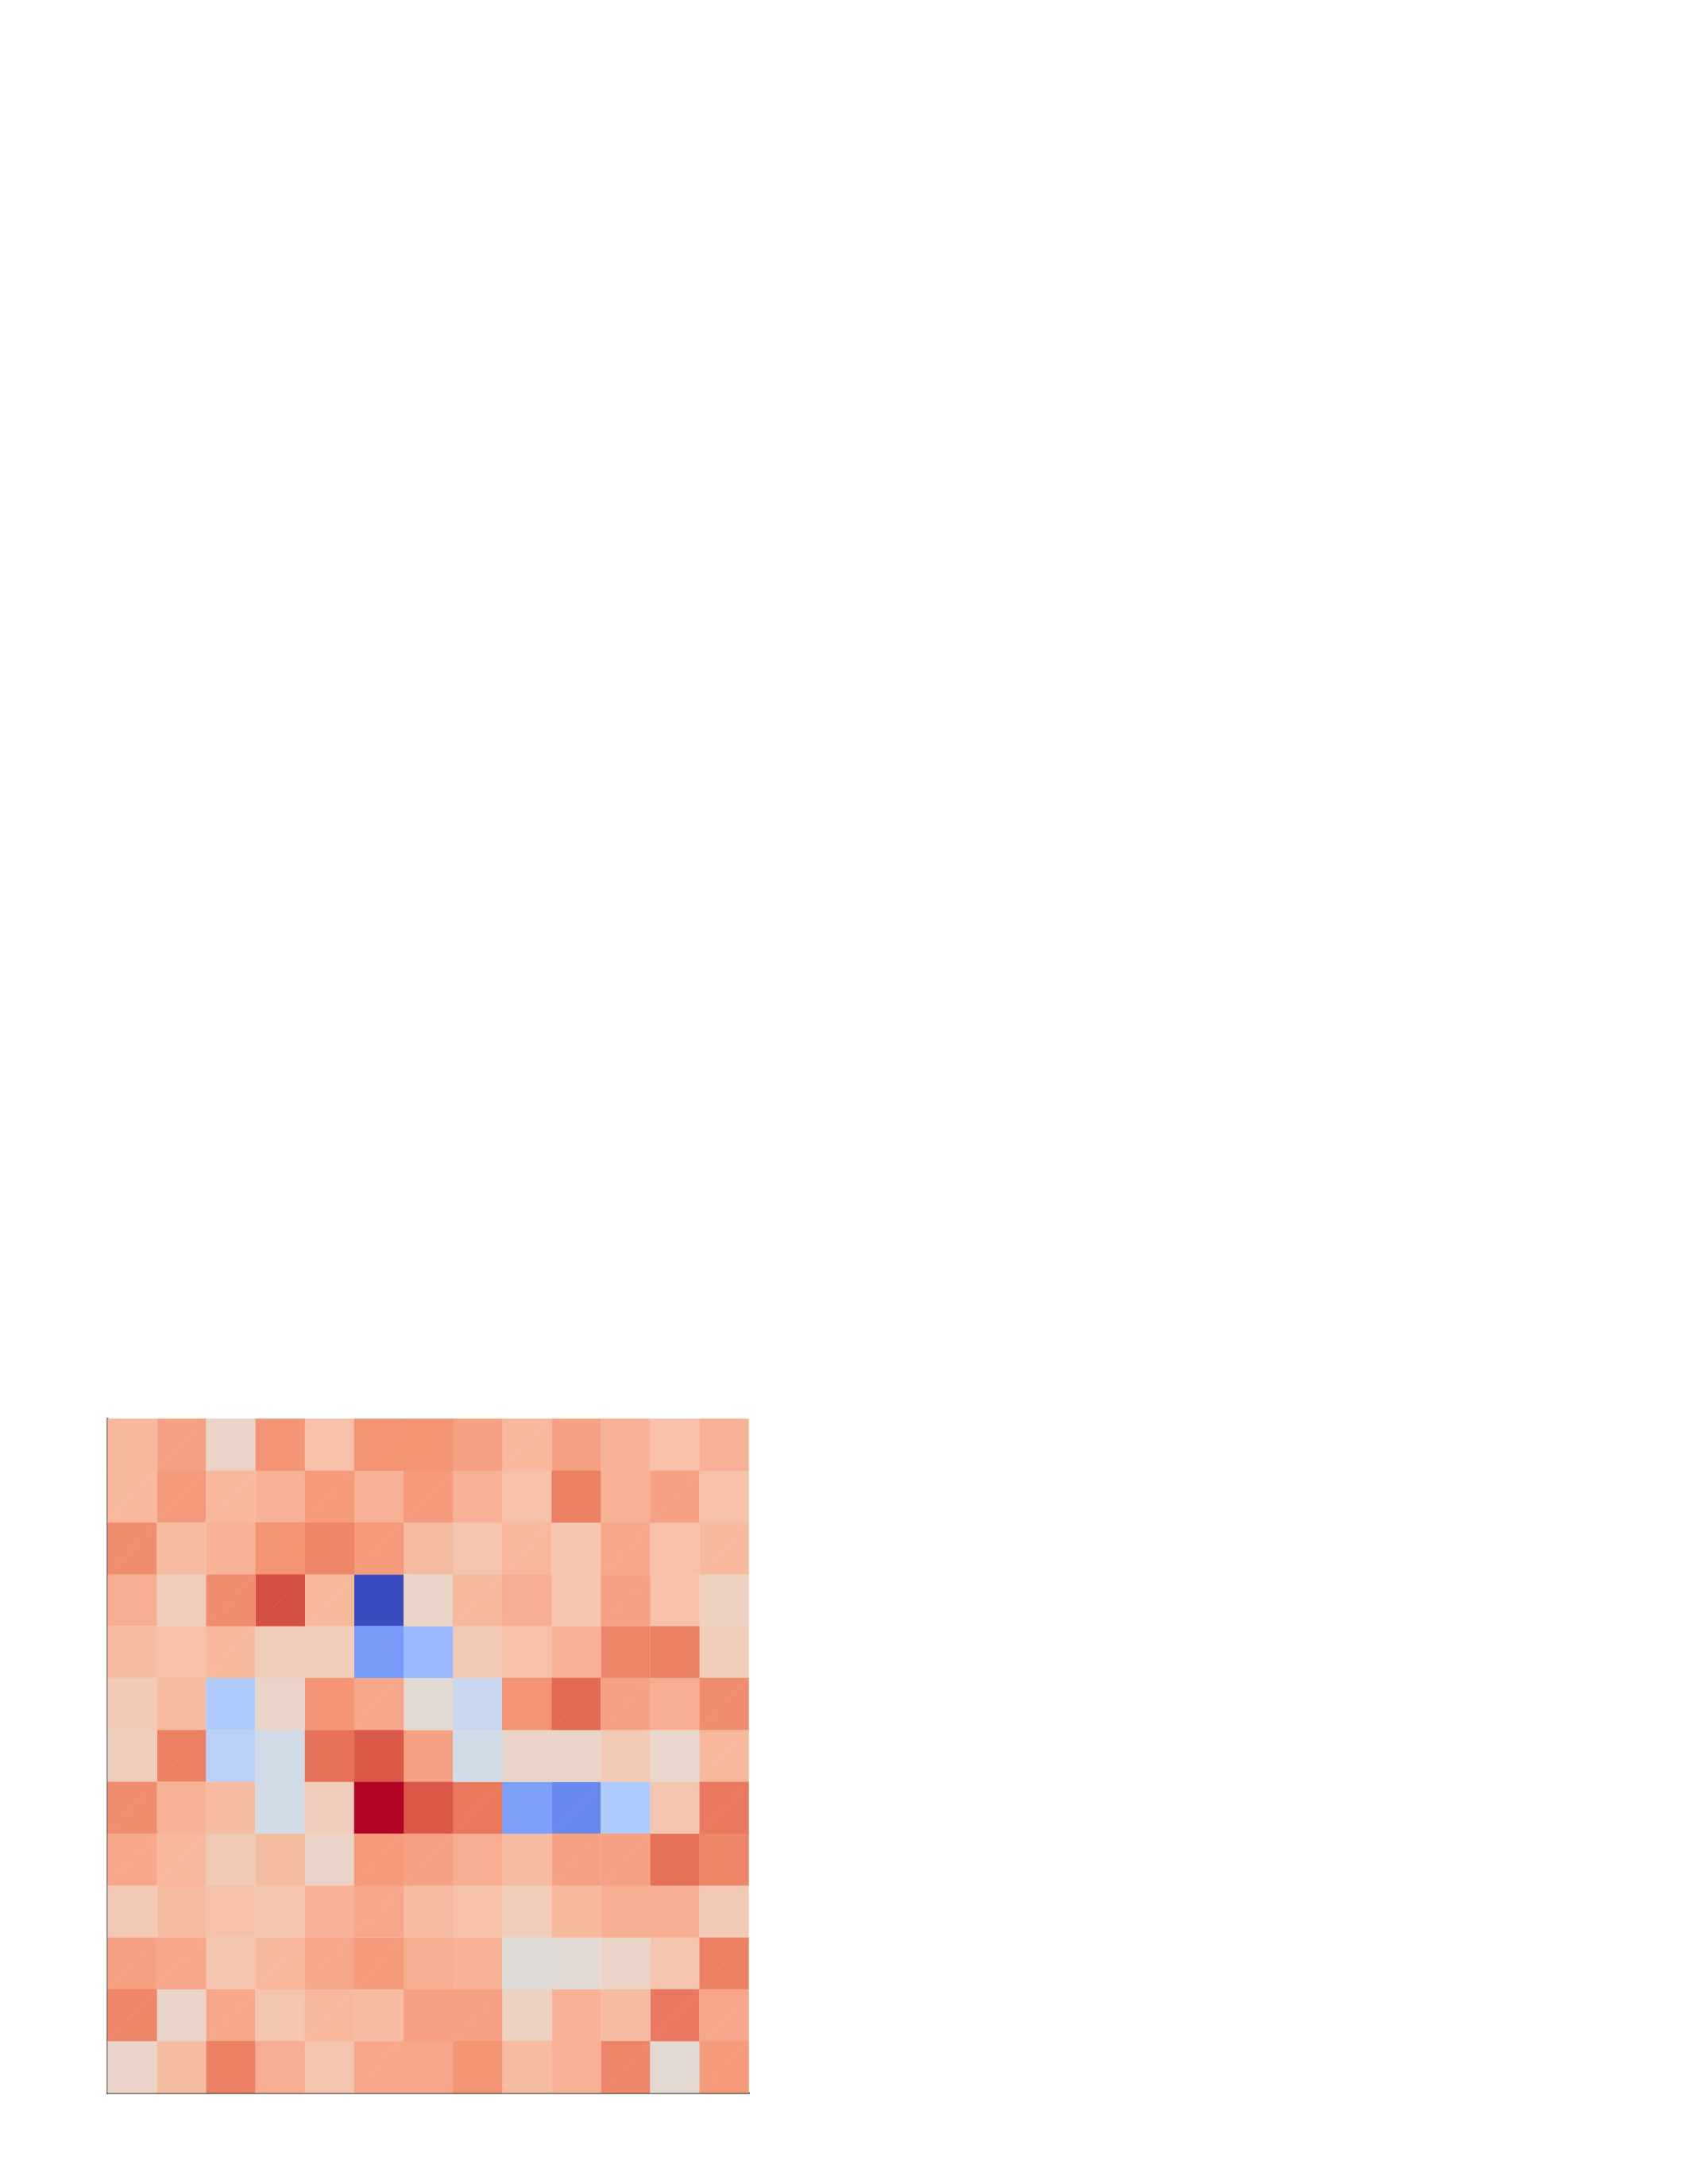}
	\includegraphics[clip = on, trim = 10mm 10mm 10mm 10mm ,width = 0.15\textwidth]{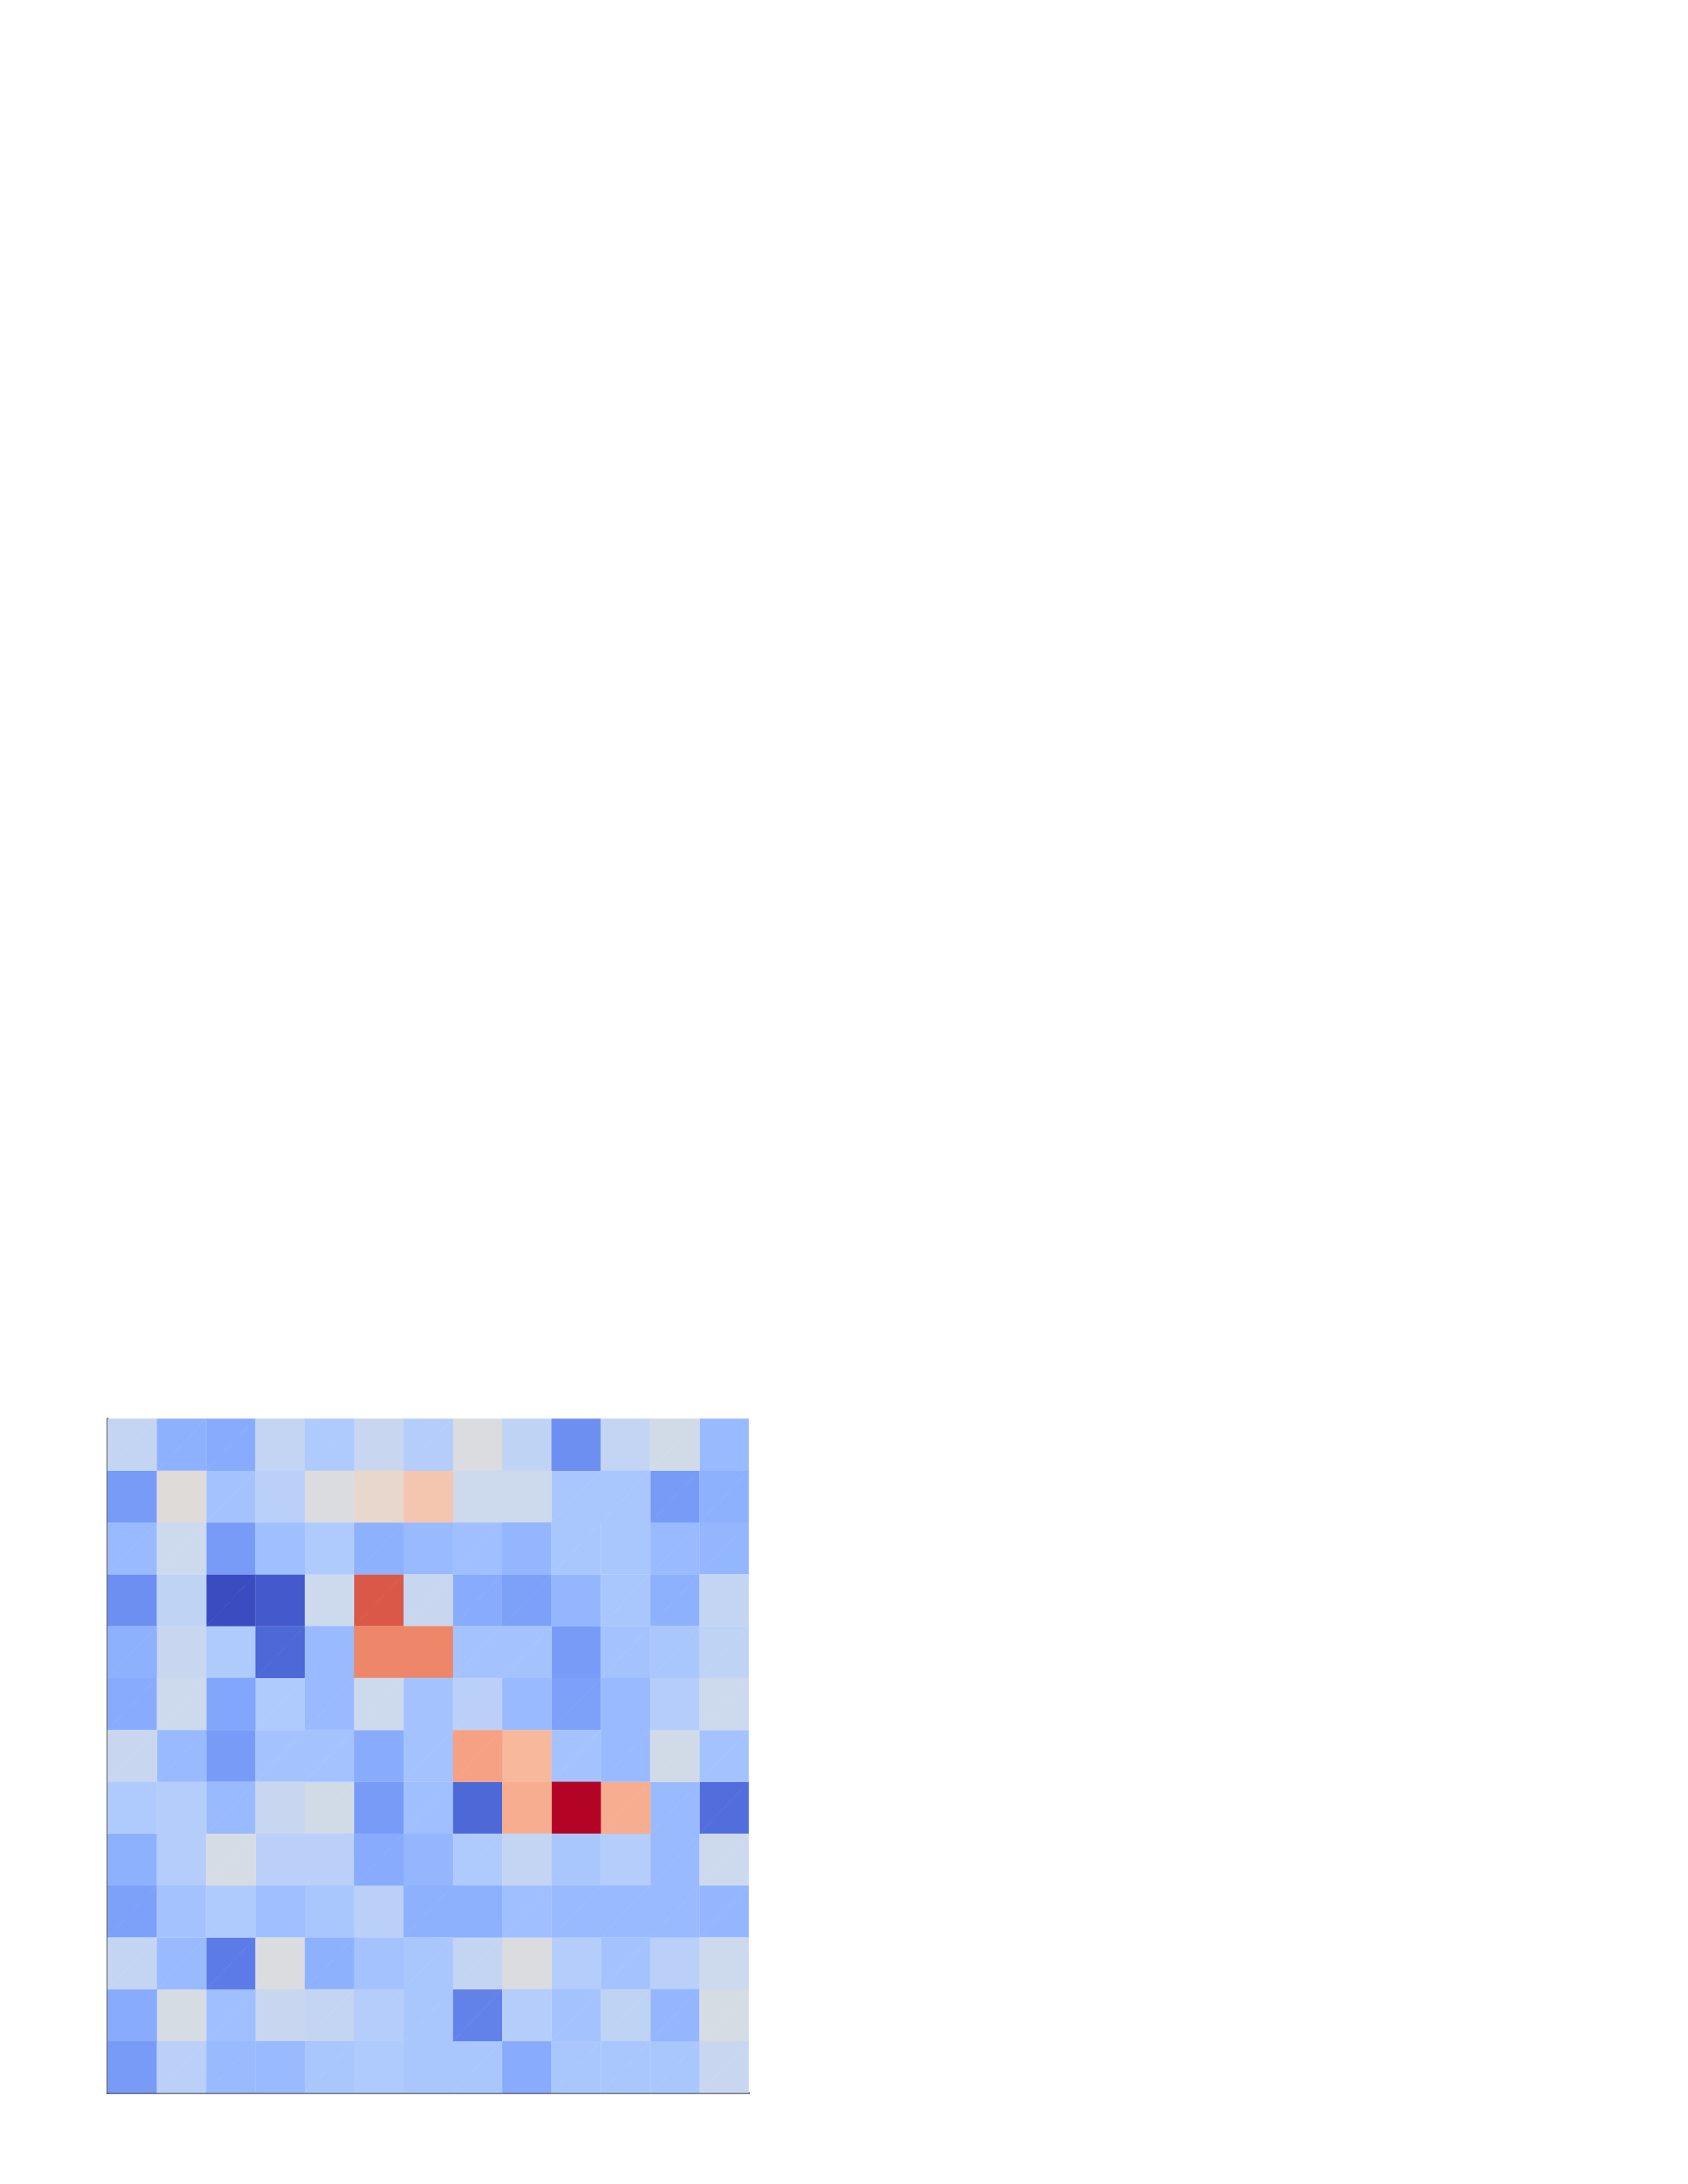} \\

	%%NEW ALTERNATIVE BRINGING ALL PIXELS BACK IN THAT HAVE A VALUE:
	\includegraphics[clip = on, trim = 10mm 10mm 10mm 10mm ,width = 0.15\textwidth]{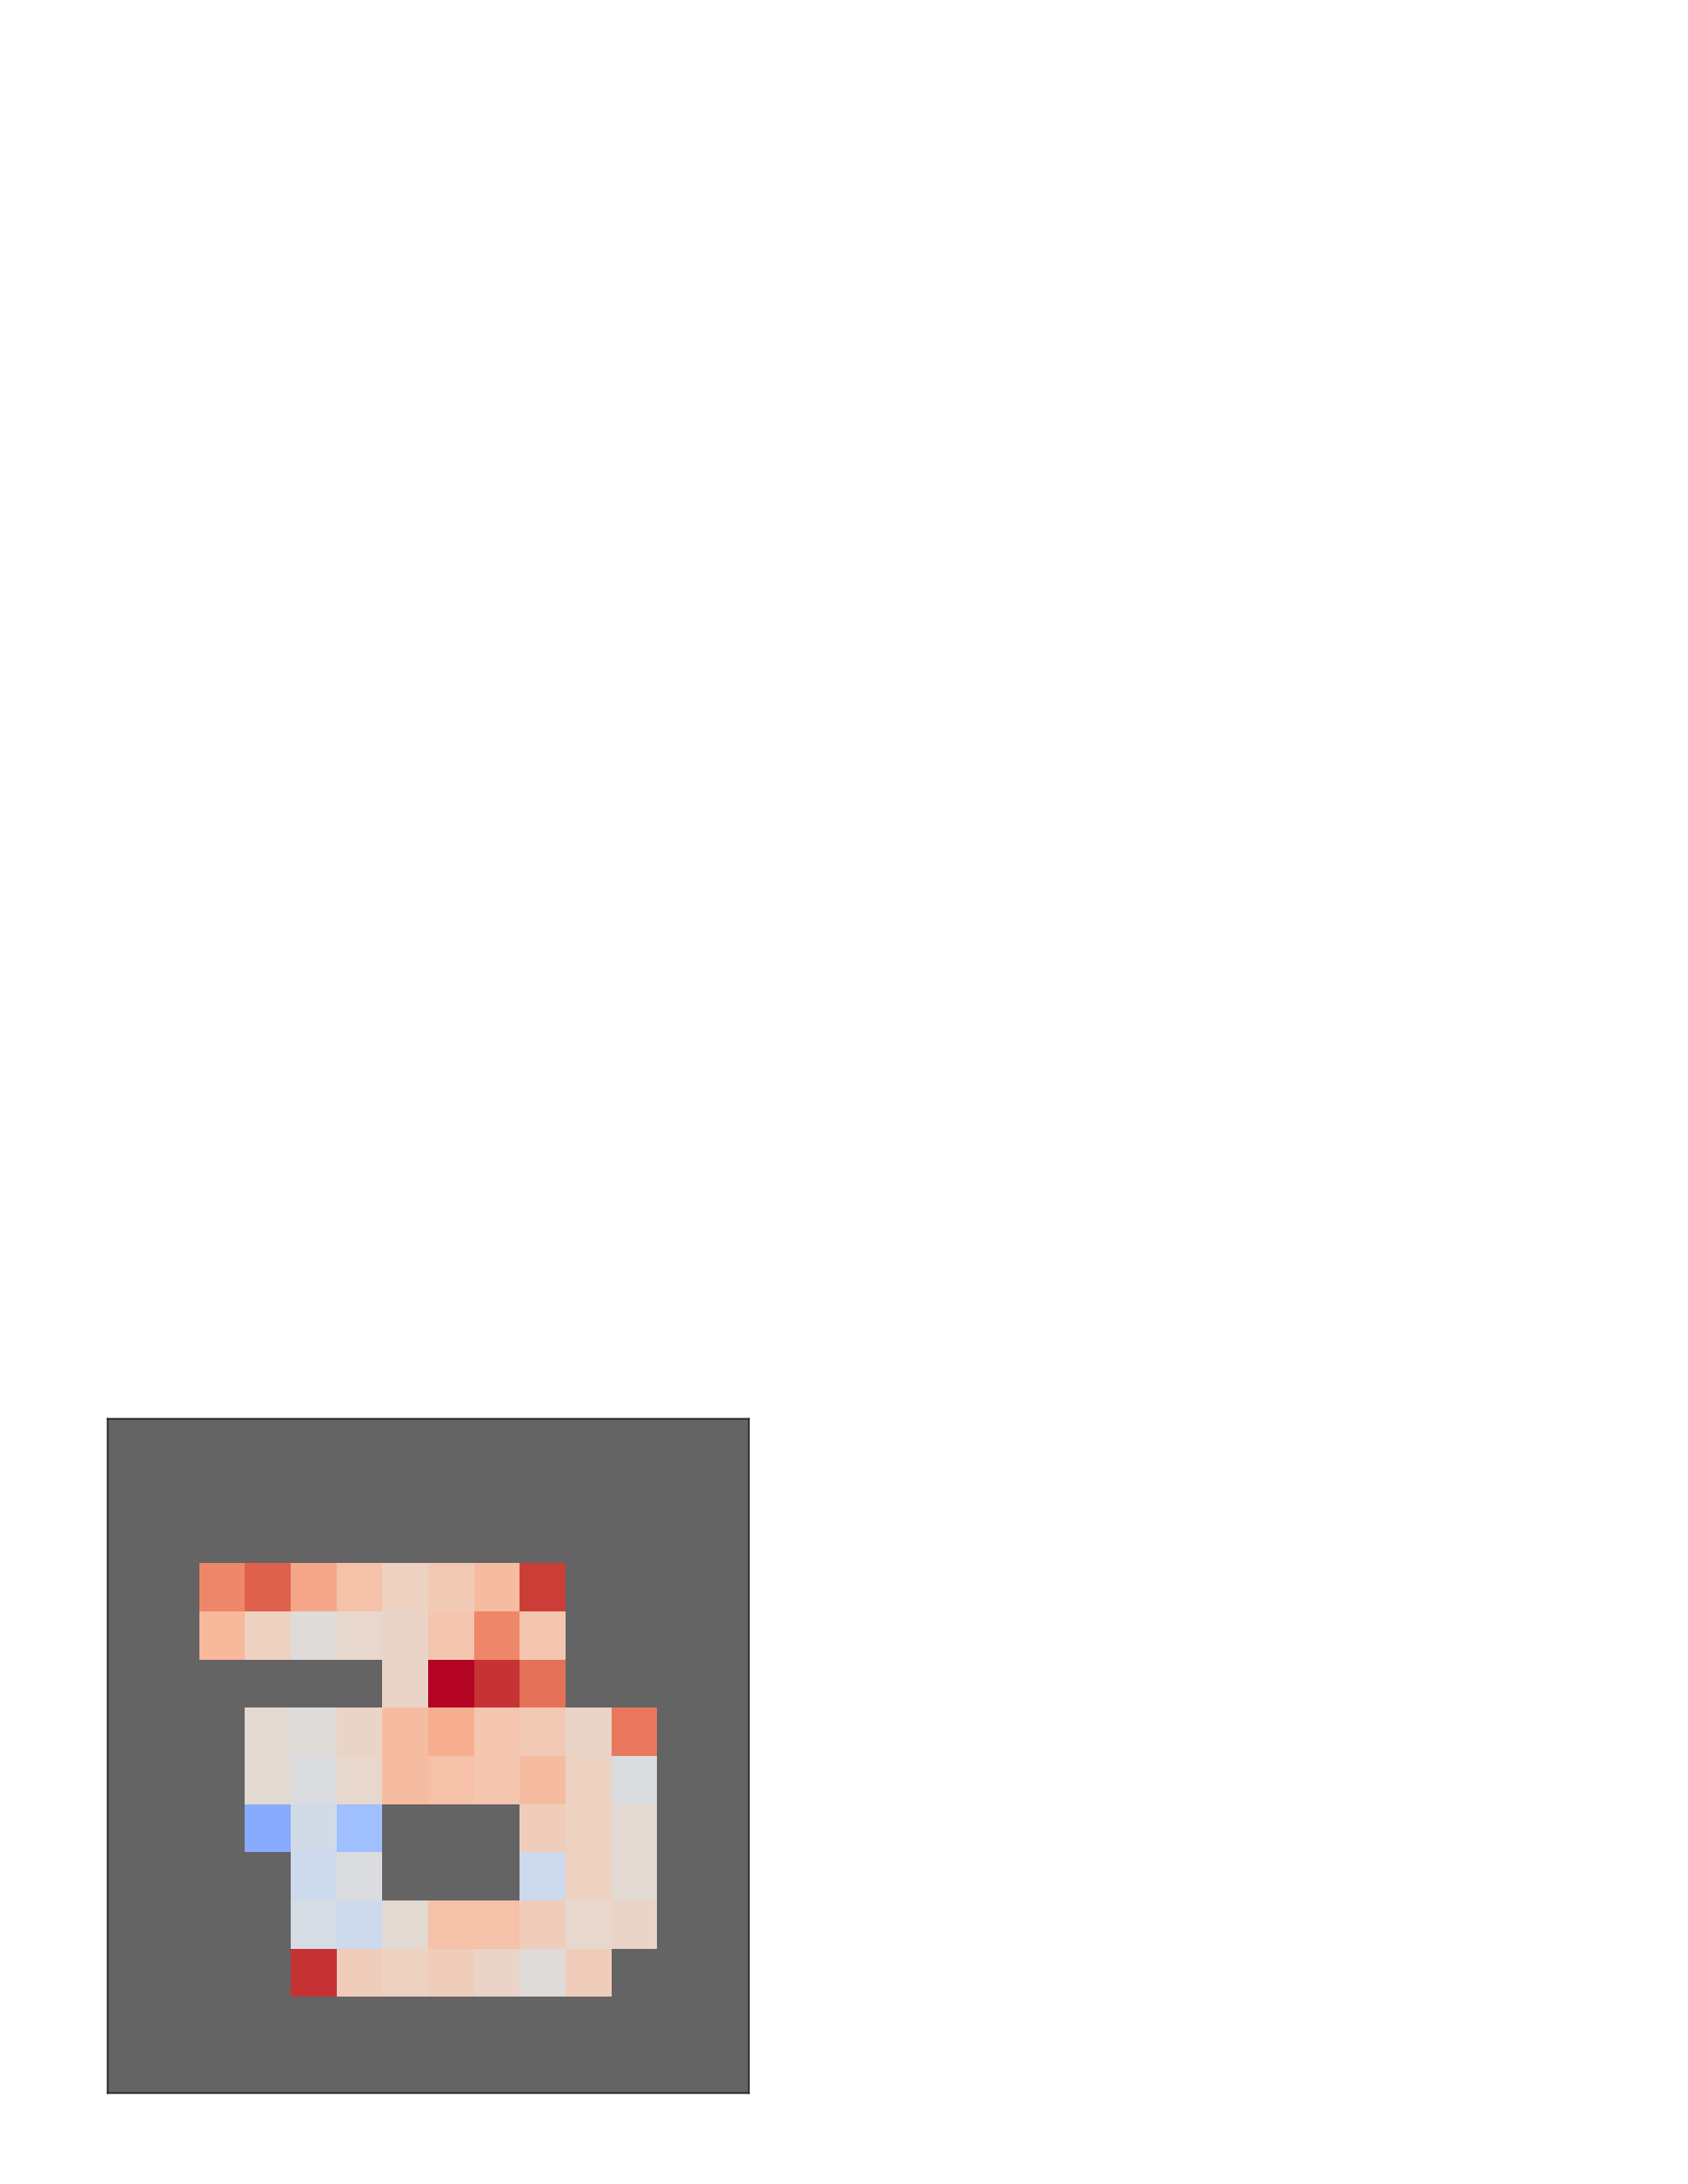}
	\includegraphics[clip = on, trim = 10mm 10mm 10mm 10mm ,width = 0.15\textwidth]{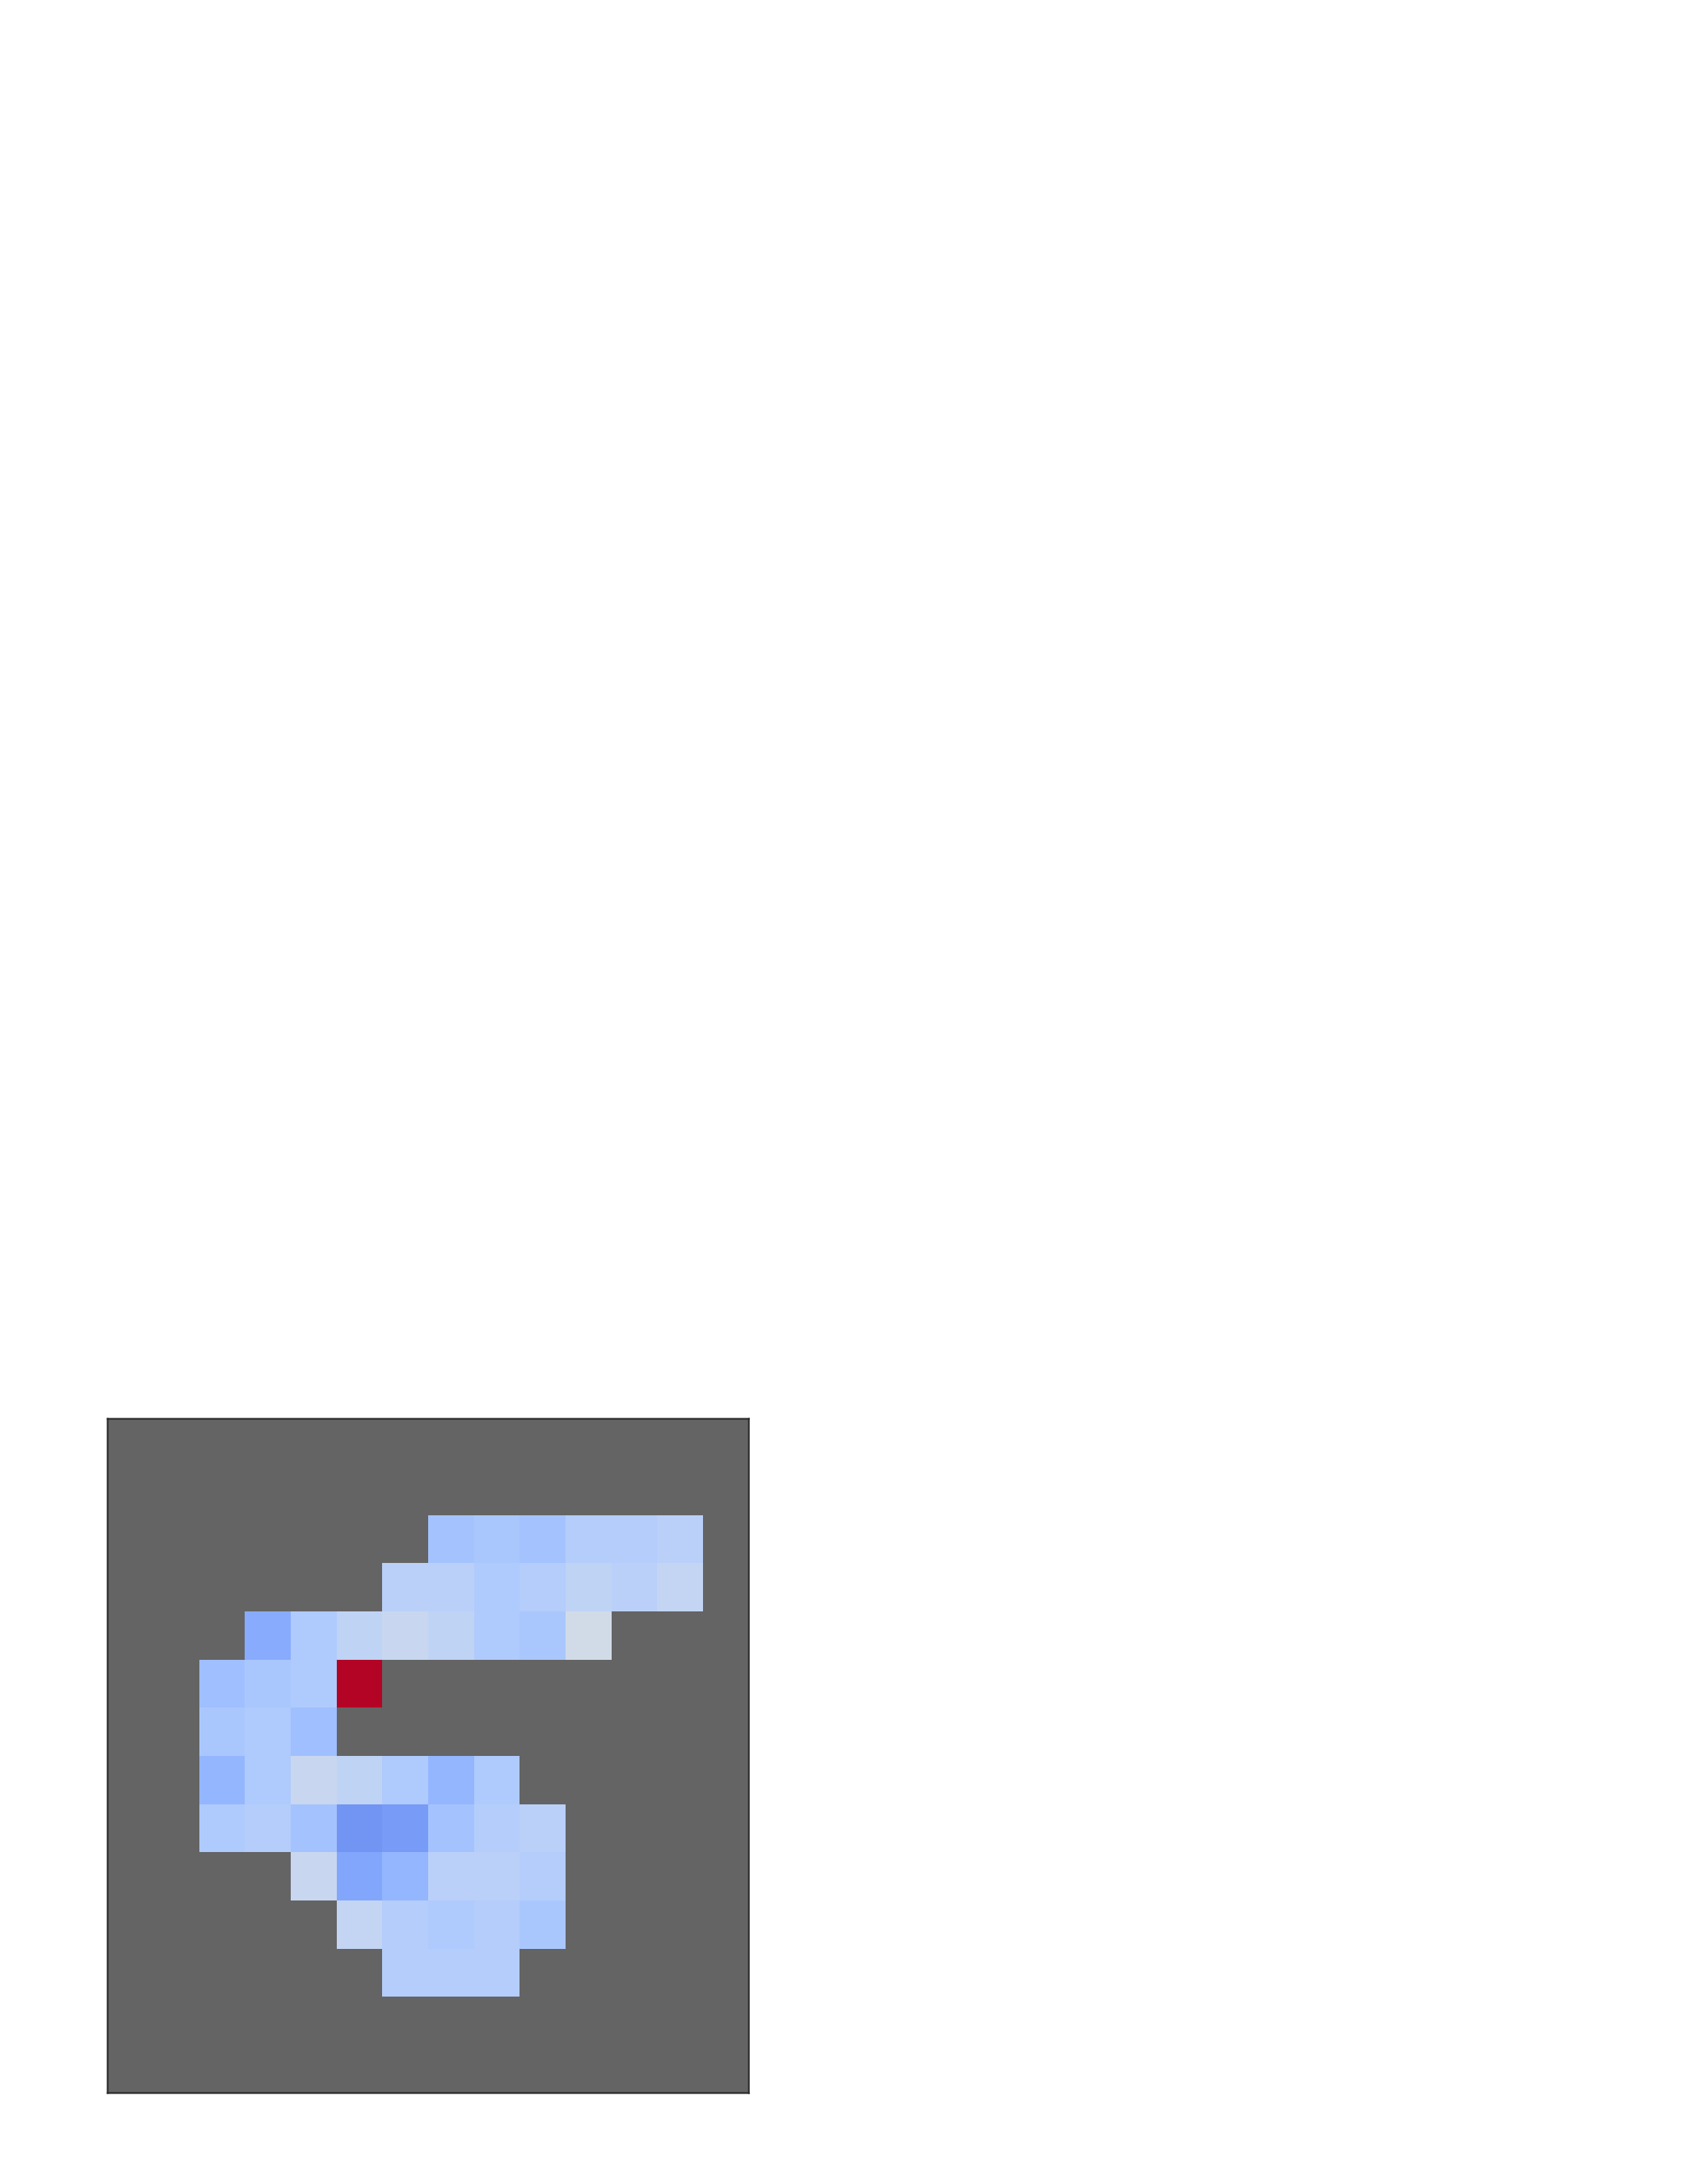}
	\includegraphics[clip = on, trim = 10mm 10mm 10mm 10mm ,width = 0.15\textwidth]{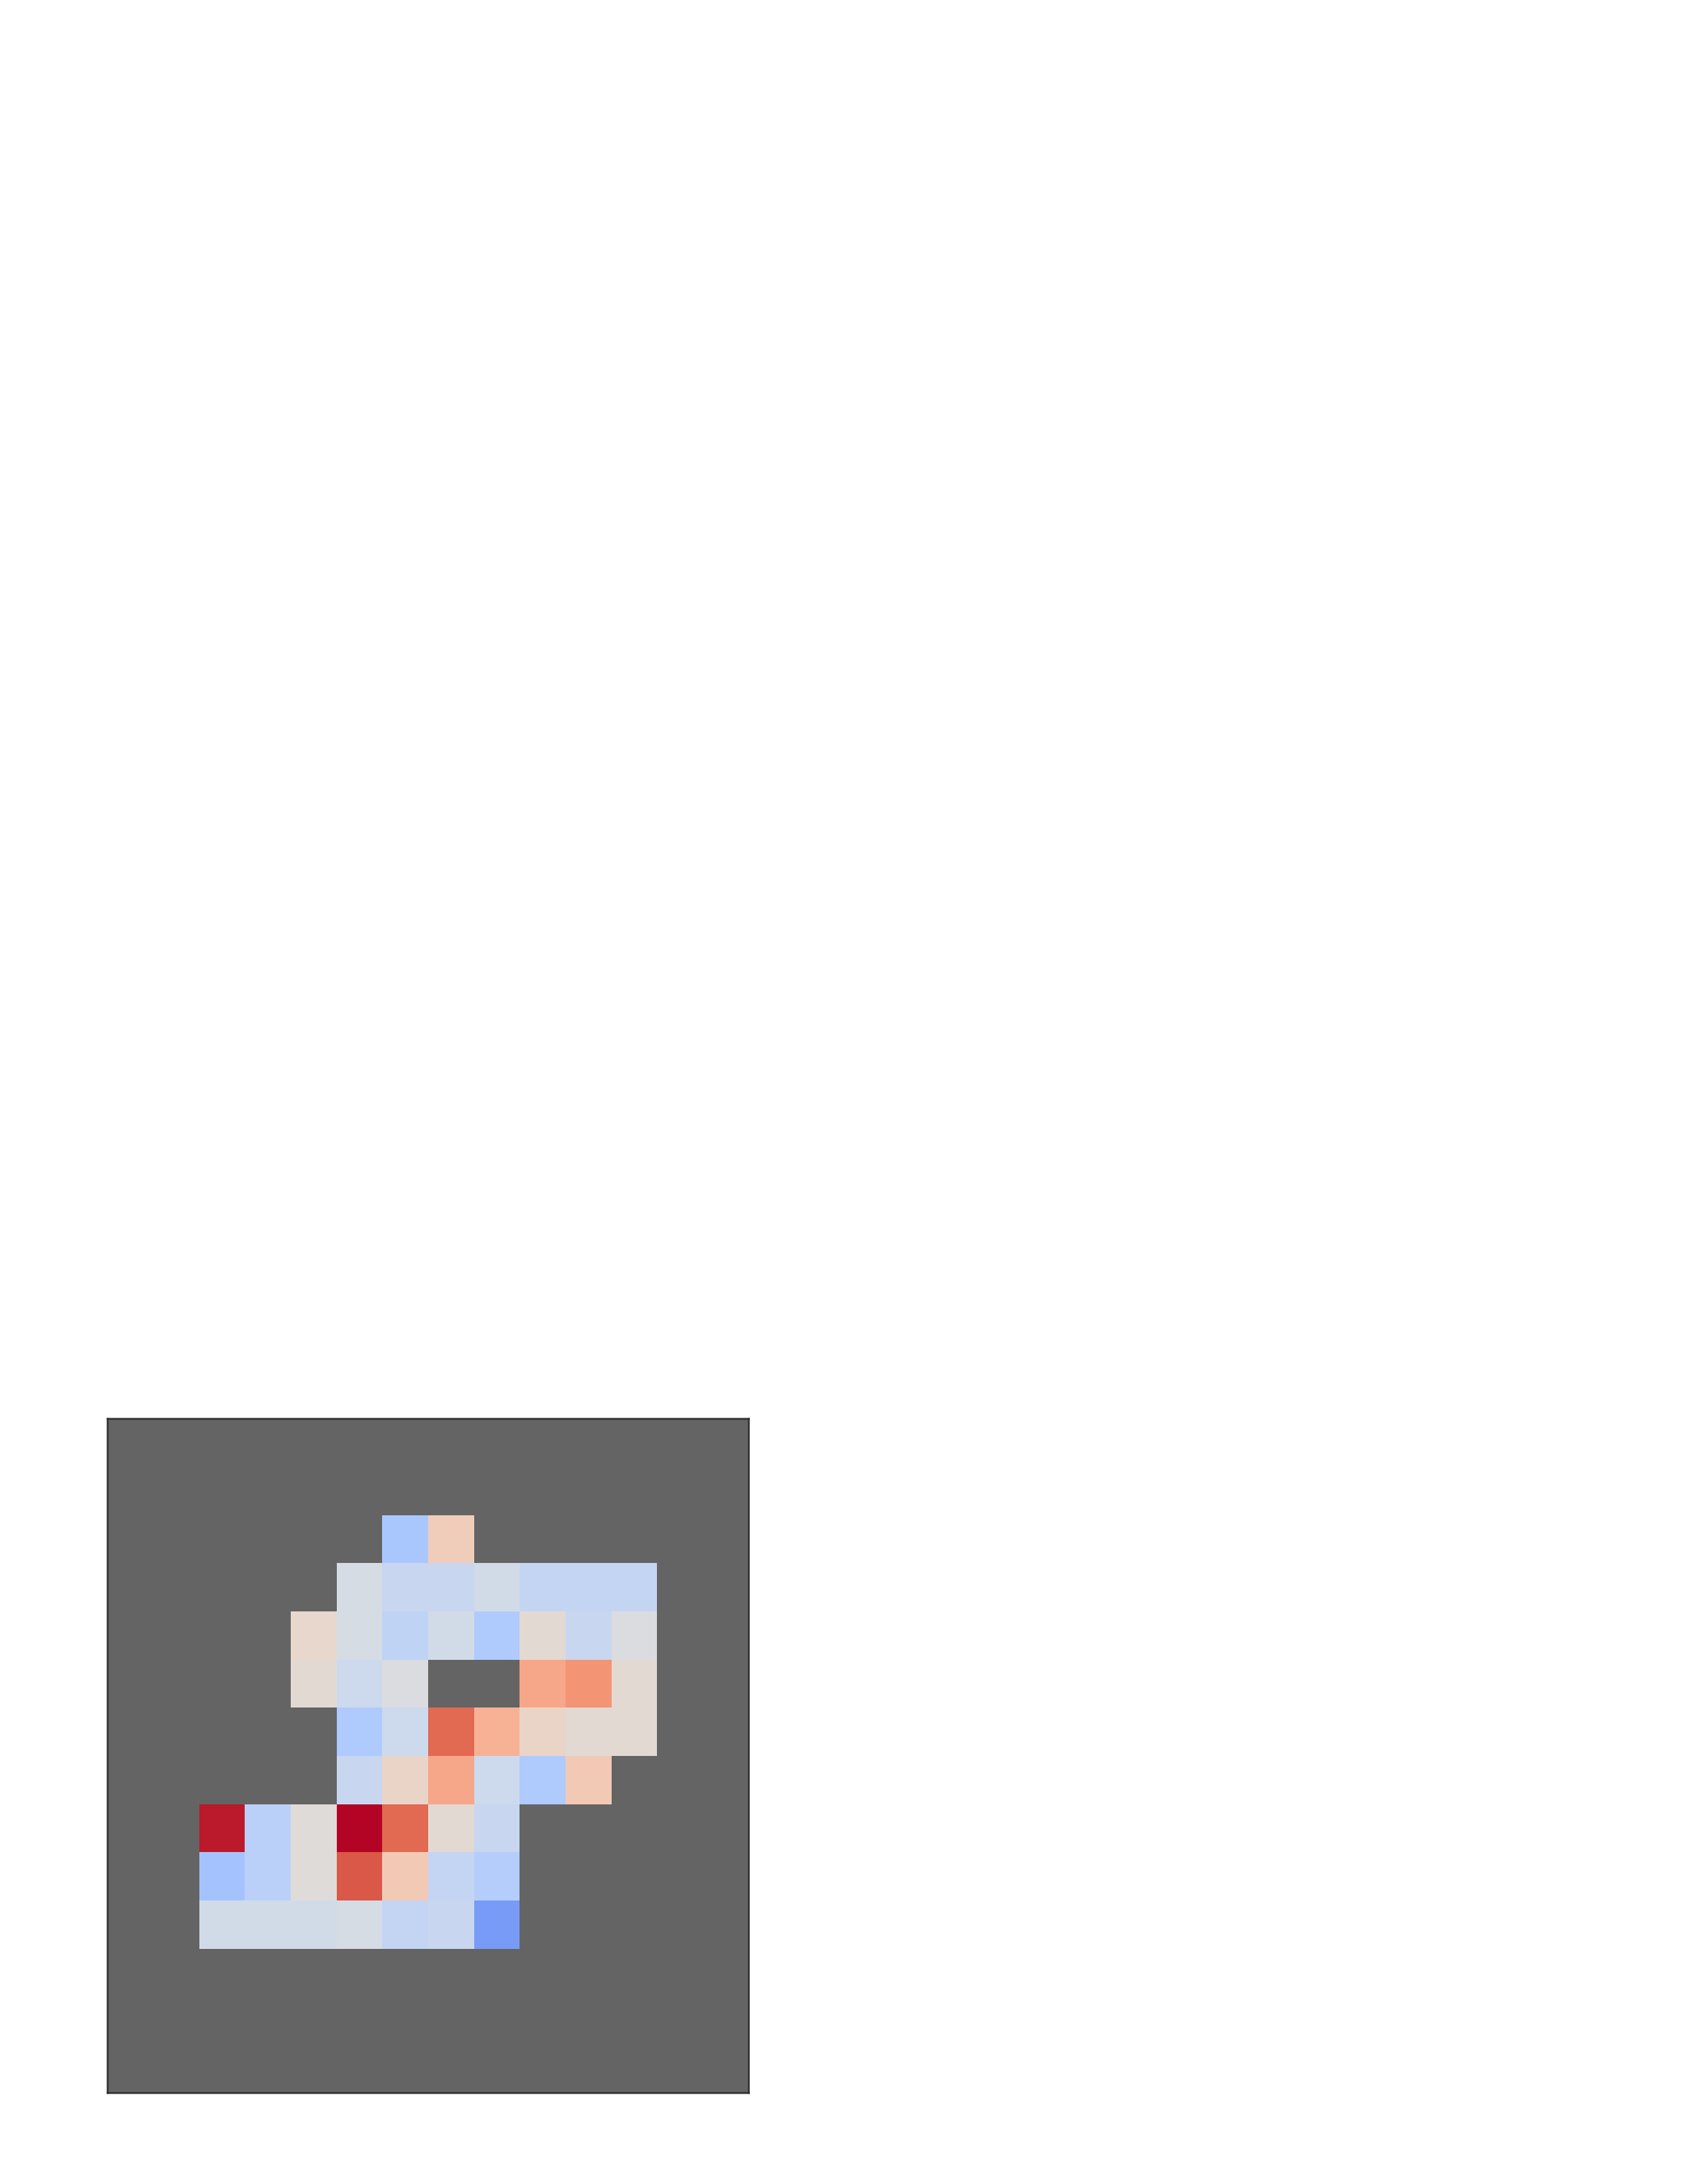}

	%%OLD VERSION, WOULD PROBABLY BRING BACK AS IT WAS NICER:
	%\includegraphics[clip = on, trim = 10mm 10mm 10mm 10mm ,width = 0.15\textwidth]{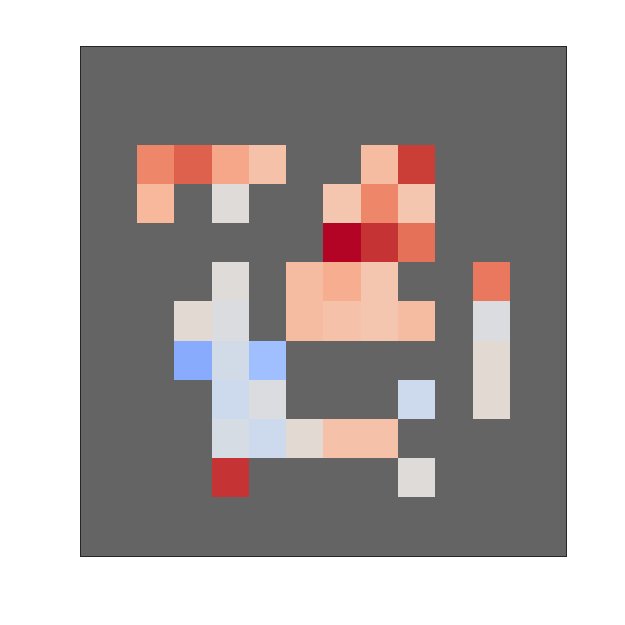}
	%\includegraphics[clip = on, trim = 10mm 10mm 10mm 10mm ,width = 0.15\textwidth]{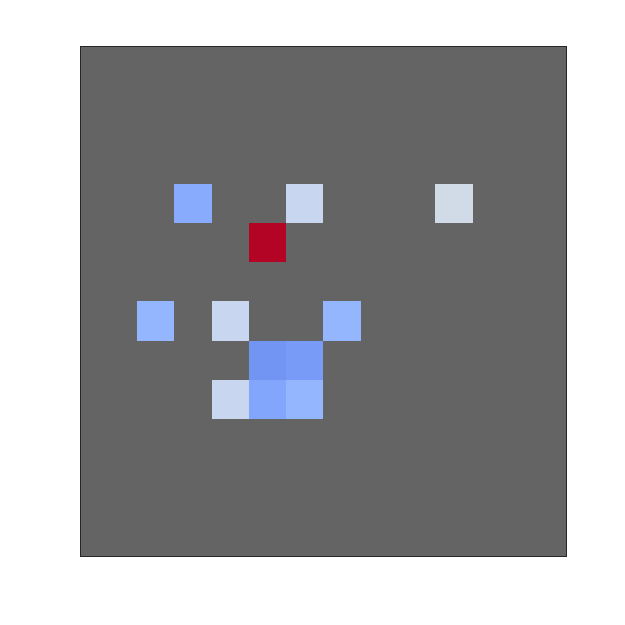}
	%\includegraphics[clip = on, trim = 10mm 10mm 10mm 10mm ,width = 0.15\textwidth]{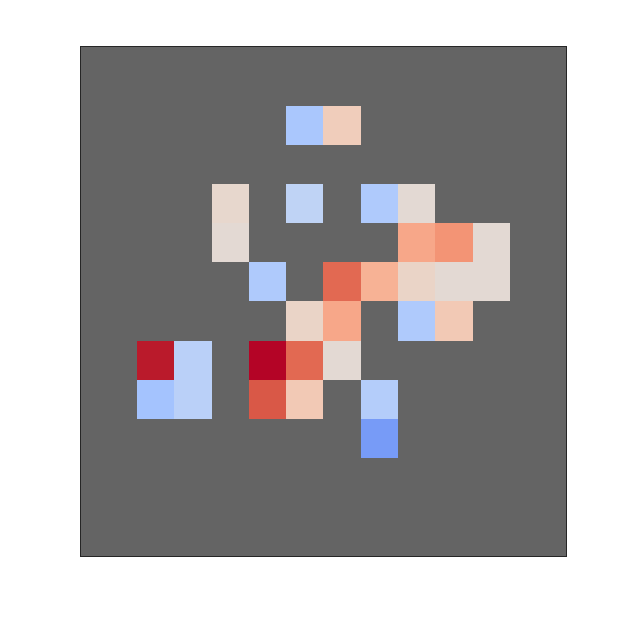}
	\caption{\textbf{First row}: Samples selected from MNIST358. \textbf{Second row}: interpretability metric estimation using our method. \textbf{Third row}: Results obtained using a LIME based approach.} 
%	\label{fig:Interpretability}
\end{wrapfigure}
